# Supplementary material for: Motif Guided Graph Transformer with Combinatorial Skeleton Prototype Learning for Skeleton-Based Person Re-Identification
Source: arXiv:2412.09044 source file (2025-02-02)
Supplement: Supplementary file 1 [file Appendix_II_Proof.pdf]

# Motif Guided Graph Transformer with Combinatorial Skeleton Prototype Learning for Skeleton-Based Person Re-Identification – Appendix II Theoretical Hypotheses and Analyses

**Haocong Rao, Chunyan Miao***

College of Computing and Data Science, Nanyang Technological University (NTU), Singapore
Joint NTU-UBC Research Centre of Excellence in Active Living for the Elderly (LILY), NTU, Singapore
{haocong001,ascymiao}@ntu.edu.sg

As our supplementary materials, we provide theoretical hypotheses and analyses of our approach in this appendix, and offer supplementary experimental settings and results in Appendix I.

The proposed combinatorial skeleton prototype learning (CSP) can be formulated as a generalized Expectation-Maximization (EM) solution. In this appendix, we first provide a theoretical EM modeling for CSP to prove its validity and convergence, and then systematically present the relations and differences between the proposed approach and existing prototype contrastive learning paradigms.

**Preliminaries.** For clarity and convenience, we adopt a more general notation here, which is different from that used in the paper. Suppose that a training set $S = \{\boldsymbol{s}_i\}_{i=1}^{N}$ contains $N$ skeleton sequences, where $\boldsymbol{s}_i \in \mathbb{R}^{F\times K}$, $K = J \times 3$, $J$ is the number of body joints with 3D positions, and $F$ is the sequence length ($i.e.$, number of consecutive skeletons). We first represent each sequence with skeleton graphs by: $G(\boldsymbol{s}_i) = \boldsymbol{x}_i = (\mathcal{G}_1, \cdots, \mathcal{G}_F)$, where $G(\cdot)$ is the *pre-defined* graph construction function, $\boldsymbol{x}_i = (\mathcal{G}_1, \cdots, \mathcal{G}_F)$ is the consecutive graphs representing the $i^{th}$ skeleton sequence $\boldsymbol{s}_i$, and $\mathcal{G}_t$ denotes the $t^{th}$ graph corresponding to the $t^{th}$ skeleton in $\boldsymbol{s}_i$. In our work, instead of using original skeleton sequences, we utilize their skeleton graph representations as inputs to capture richer skeletal body and motion features. The objective of skeleton graph representation learning is to learn a graph embedding/encoder function $f_\theta$ (realized via $\theta$-parameterized neural networks) that maps the skeleton graphs $\boldsymbol{x}_i$ to $\boldsymbol{v}_i \in \mathbb{R}^H$, by $\boldsymbol{v}_i = f_\theta(\boldsymbol{x}_i)$, such that $\boldsymbol{v}_i$ can effectively represent latent features of $\boldsymbol{x}_i$ to perform person re-identification.

Formally, the goal is to find the network parameter $\theta$ that maximizes the log-likelihood function of the observed graph representations $\{\boldsymbol{x}_i\}_{i=1}^{N}$ of $N$ skeleton sequences as follows:

$$\begin{aligned}\theta^* &= \arg\max_\theta L(\boldsymbol{x}_1, \cdots, \boldsymbol{x}_N; \theta) \\ &= \arg\max_\theta \prod_{i=1}^{N} p(\boldsymbol{x}_i; \theta) \\ &\iff \arg\max_\theta \sum_{i=1}^{N} \log p(\boldsymbol{x}_i; \theta), \end{aligned} \tag{1}$$

where $L(\boldsymbol{x}_1, \cdots, \boldsymbol{x}_N; \theta)$ denotes the likelihood function of the observed skeleton graph representations *with regard to* $\theta$, and each skeleton graph representation $\boldsymbol{x}_i$ is hypothetically related to a certain skeleton prototype[1] $\boldsymbol{c}_j \in \mathbb{R}^H$, with $\boldsymbol{c}_j \in \{\boldsymbol{c}_j\}_{j=1}^{K}$ and $K$ is the number of skeleton prototypes. Under this assumption, we can re-formulate the objective in Eq. (1) as:

$$\begin{aligned}\theta^* =& \arg\max_\theta \sum_{i=1}^{N} \log p(\boldsymbol{x}_i; \theta) \\ =& \arg\max_\theta \sum_{i=1}^{N} \log \sum_{j=1}^{K} p(\boldsymbol{x}_i, \boldsymbol{c}_j; \theta), \end{aligned} \tag{2}$$

Directly optimizing this function is intractable, thus we consider a lower-bound by using a surrogate function as:

$$\begin{aligned}&\sum_{i=1}^{N} \log \sum_{j=1}^{K} p(\boldsymbol{x}_i, \boldsymbol{c}_j; \theta) \\ =& \sum_{i=1}^{N} \log \sum_{j=1}^{K} Q(\boldsymbol{c}_j) \frac{p(\boldsymbol{x}_i, \boldsymbol{c}_j; \theta)}{Q(\boldsymbol{c}_j)} \\ \geq& \sum_{i=1}^{N} \sum_{j=1}^{K} Q(\boldsymbol{c}_j) \log \frac{p(\boldsymbol{x}_i, \boldsymbol{c}_j; \theta)}{Q(\boldsymbol{c}_j)}, \end{aligned} \tag{3}$$

where $Q(\boldsymbol{c}_j)$ represents some distribution over $\{\boldsymbol{c}_j\}_{j=1}^{K}$ and $\sum_{j=1}^{K} Q(\boldsymbol{c}_j) = 1$. We apply Jensen's inequality to derive

*Corresponding author
Copyright © 2025, Association for the Advancement of Artificial Intelligence (www.aaai.org). All rights reserved.

[1]For simplicity of presentation, we use "skeleton graph representation" to denote the graph representation of a skeleton sequence, and use "skeleton prototype" to denote the prototype of skeleton graph representations.

the last step of Eq. (3), where the equality can be achieved under the condition that $\frac{p(\boldsymbol{x}_i, \boldsymbol{c}_j; \theta)}{Q(\boldsymbol{c}_j)}$ is a constant. To realize this equality, we have:

$$Q\left(\boldsymbol{c}_j\right) = \frac{p\left(\boldsymbol{x}_i, \boldsymbol{c}_j; \theta\right)}{\sum_{m=1}^{K} p\left(\boldsymbol{x}_i, \boldsymbol{c}_m; \theta\right)} = \frac{p\left(\boldsymbol{x}_i, \boldsymbol{c}_j; \theta\right)}{p\left(\boldsymbol{x}_i; \theta\right)} = p\left(\boldsymbol{c}_j; \boldsymbol{x}_i, \theta\right), \quad (4)$$

where $Q\left(\boldsymbol{c}_j\right)$ is a posterior probability related to $\boldsymbol{c}_j, \boldsymbol{x}_i$, and $\theta$. Different from (Rao and Miao 2022; Rao and Miao 2022; Rao, Leung, and Miao 2024) that employ clustering to estimate prototypes and representation distributions under the fixed $\theta$, we exploit the graph feature centroid of each *ground-truth* identity as a different skeleton prototype. In particular, when given the $\theta$-parameterized encoder to encode all skeleton graphs ($\boldsymbol{x}_i$) *at the Expectation step*, their corresponding prototypes ($\boldsymbol{c}_j$) are assumed to follow the distribution of ground-truth classes in the dataset. The skeleton prototype distribution is hence constant and can be computed by $Q\left(\boldsymbol{c}_j\right) = p\left(\boldsymbol{c}_j; \boldsymbol{x}_i, \theta\right)$. We can re-write Eq. (3) as:

$$\sum_{i=1}^{N} \sum_{j=1}^{K} \left(Q\left(\boldsymbol{c}_j\right) \log p\left(\boldsymbol{x}_i, \boldsymbol{c}_j; \theta\right) - Q\left(\boldsymbol{c}_j\right) \log Q\left(\boldsymbol{c}_j\right)\right), \quad (5)$$

where the constant $-\sum_{i=1}^{N} \sum_{j=1}^{K} Q\left(\boldsymbol{c}_j\right) \log Q\left(\boldsymbol{c}_j\right)$ can be ignored and we need to maximize:

$$\sum_{i=1}^{N} \sum_{j=1}^{K} Q\left(\boldsymbol{c}_j\right) \log p\left(\boldsymbol{x}_i, \boldsymbol{c}_j; \theta\right). \quad (6)$$

For **the Expectation (E)-step**, $p\left(\boldsymbol{c}_j; \boldsymbol{x}_i, \theta\right)$ (see Eq. (4)) is estimated by the ground-truth class distribution. In our approach, the number of skeleton prototypes ($K$) is identical to the number of different classes, and we generate skeleton prototypes $\{\boldsymbol{c}_j\}_{j=1}^{K}$ by computing the feature *centroids* of *encoded* skeleton graph representations $\boldsymbol{v}_i$ in different classes. We use $\{\boldsymbol{C}_j\}_{j=1}^{K}$ to denote the groups[2] of graph representations (referred to as *"sample groups"*) belonging to different prototypes. Then, we compute $p\left(\boldsymbol{c}_j; \boldsymbol{x}_i, \theta\right) = \mathbb{1}\left(\boldsymbol{x}_i \in \boldsymbol{C}_j\right)$, where $\mathbb{1}\left(\boldsymbol{x}_i \in \boldsymbol{C}_j\right) = 1$ if $\boldsymbol{x}_i$ belongs to the $j^{th}$ sample group $\boldsymbol{C}_j$ (*i.e.*, belonging to skeleton prototype $\boldsymbol{c}_j$); otherwise $\mathbb{1}\left(\boldsymbol{x}_i \in \boldsymbol{C}_j\right) = 0$.

**Assumption 1** ***Prototype-Class Consistency.*** *The global distribution of skeleton prototypes is consistent with the distribution of class feature centroids, i.e., all samples belonging to a ground-truth class explicitly correspond to the sample group of a certain prototype. In the E-step, we adopt this assumption to generate skeleton prototypes and derive* $p\left(\boldsymbol{c}_j; \boldsymbol{x}_i, \theta\right) = \mathbb{1}\left(\boldsymbol{x}_i \in \boldsymbol{C}_j\right)$.

In the **Maximization (M)-step**, we combine Eq. (4) to maximize the lower-bound in Eq. (6) after the E-step:

$$\begin{aligned} &\sum_{i=1}^{N} \sum_{j=1}^{K} Q\left(\boldsymbol{c}_j\right) \log p\left(\boldsymbol{x}_i, \boldsymbol{c}_j; \theta\right) \\ &= \sum_{i=1}^{N} \sum_{j=1}^{K} p\left(\boldsymbol{c}_j; \boldsymbol{x}_i, \theta\right) \log p\left(\boldsymbol{x}_i, \boldsymbol{c}_j; \theta\right) \\ &= \sum_{i=1}^{N} \sum_{j=1}^{K} \mathbb{1}\left(\boldsymbol{x}_i \in \boldsymbol{C}_j\right) \log p\left(\boldsymbol{x}_i, \boldsymbol{c}_j; \theta\right). \end{aligned} \quad (7)$$

Assumed that each class is equally important and the sample number of each class is approximately identical in learning, each skeleton prototype $\boldsymbol{c}_j$ can have a uniform prior probability $p\left(\boldsymbol{c}_j; \theta\right) = \frac{1}{K}$. We have:

$$\begin{aligned} p\left(\boldsymbol{x}_i, \boldsymbol{c}_j; \theta\right) &= p\left(\boldsymbol{x}_i; \boldsymbol{c}_j, \theta\right) p\left(\boldsymbol{c}_j; \theta\right) \\ &= \frac{1}{K} \cdot p\left(\boldsymbol{x}_i; \boldsymbol{c}_j, \theta\right), \end{aligned} \quad (8)$$

where the distribution of samples around each skeleton prototype is assumed to be an isotropic Gaussian, leading to:

$$p\left(\boldsymbol{x}_i; \boldsymbol{c}_j, \theta\right) = \frac{\exp\left(\frac{-(\boldsymbol{v}_i - \boldsymbol{c}_p)^2}{2\sigma_p^2}\right)}{\sum_{j=1}^{K} \exp\left(\frac{-(\boldsymbol{v}_i - \boldsymbol{c}_j)^2}{2\sigma_j^2}\right)}, \quad (9)$$

where $\boldsymbol{v}_i = f_\theta\left(\boldsymbol{x}_i\right)$ and $\boldsymbol{c}_p$ is the skeleton prototype for the sample group $\boldsymbol{C}_p$ containing $\boldsymbol{x}_i$, *i.e.*, $\boldsymbol{x}_i \in \boldsymbol{C}_p$. We apply $\ell_2$-normalization to both $\boldsymbol{v}$ and $\boldsymbol{c}$ to have $(\boldsymbol{v} - \boldsymbol{c})^2 = 2 - 2\boldsymbol{v} \cdot \boldsymbol{c}$. Then combining this with Eq. (2), (3), (6), (7), (8), and (9), we can get the maximum log-likelihood estimation with:

$$\theta^* = \arg\min_{\theta} \sum_{i=1}^{N} -\log \frac{\exp\left(\boldsymbol{v}_i \cdot \boldsymbol{c}_p / \tau_p\right)}{\sum_{j=1}^{K} \exp\left(\boldsymbol{v}_i \cdot \boldsymbol{c}_j / \tau_j\right)}, \quad (10)$$

where $\boldsymbol{v}_i$ denotes the encoded features of $i^{th}$ sample (*i.e.*, skeleton graph representation) belonging to the skeleton prototype $\boldsymbol{c}_p$, and the factor $\tau$ (termed temperature) is related to the distribution of encoded graph representations around different skeleton prototypes.

**Assumption 2** ***Maximum Homogeneous Similarity.*** *The homogeneous samples, which are defined as samples within the same-prototype sample group, should share higher inherent similarity than heterogeneous samples between different groups. In other words, the skeleton prototype of each sample group can represent the unique skeleton concepts and attributes of a certain identity, and the same group's samples possess the homogeneity of features corresponding to this prototype (Nauta et al. 2022). According to Assumption 1, it can be equivalent to the objective that the representation of each sample should be maximally similar to the corresponding prototype and be minimally similar to other prototypes. In the M-step, we maximize the probability that each sample representation belongs to its unique prototype (see Eq. (9)) based on this assumption. The equivalent formulation of this objective in Eq. (10) after applying feature* $\ell_2$*-normalization can be further interpreted as to maximize the dot-product based similarity between samples and their prototypes while maximizing the dissimilarity to other prototypes.*

[2] The skeleton prototypes $\{\boldsymbol{c}_j\}_{j=1}^{K}$ for $\{\boldsymbol{x}_i\}_{i=1}^{N}$ are generated based on their encoded features $\{\boldsymbol{v}_i\}_{i=1}^{N}$, while $\{\boldsymbol{C}_j\}_{j=1}^{K}$ are groups of $\{\boldsymbol{x}_i\}_{i=1}^{N}$ belonging to different skeleton prototypes.

**Relations to Existing Contrastive Learning Losses (van den Oord, Li, and Vinyals 2018; He et al. 2020; Chen et al. 2020; Li et al. 2021):**

- The InfoNCE loss (van den Oord, Li, and Vinyals 2018) re-formulated in MoCo (He et al. 2020) and SimCLR (Chen et al. 2020) can be interpreted as special cases of the maximum log-likelihood estimation in Eq. (10), where the prototype $\boldsymbol{c}_p$ for a feature $\boldsymbol{v}_i$ is replaced by the augmented feature $\boldsymbol{v'}_i$ generated from different views of augmentation of the same instance ($i.e.$, $\boldsymbol{c}_p = \boldsymbol{v'}_i$) and the temperature $\tau$ is empirically fixed for contrastive learning.
- The ProtoNCE loss used in PCL (Li et al. 2021) is a combination of momentum-based contrastive learning (He et al. 2020) and unsupervised prototype estimation with $k$-means clustering. It has a similar form as Eq. (10), where $\tau$ is estimated with the assumption that the distribution of feature representations around each prototype varies in different clusters. However, PCL estimates the feature distribution under the Euclidean distance metric used in the $k$-means clustering. Such estimation could be inapplicable ($e.g.$, can not be generalized) to models that employ different clustering algorithms ($e.g.$, density-based DBSCAN (Ester et al. 1996)) or/and different distance metrics ($e.g.$, Jaccard metric), thus failing to getting satisfactory performance in practice (Rao and Miao 2022).

**Relations to Existing Skeleton Prototype Learning Losses (Rao and Miao 2022; Rao and Miao 2022; Rao, Leung, and Miao 2024; Rao and Miao 2023):**

- The skeleton sequence prototype contrastive (SPC) loss in (Rao and Miao 2022), masked prototype contrastive (MPC) loss in (Rao and Miao 2022), and hierarchical meta-prototype contrastive (Hi-MPC) loss in (Rao, Leung, and Miao 2024) can be viewed as *unsupervised* generalized versions of the objective in Eq. (10). ALL of them leverage unsupervised clustering algorithms ($e.g.$, DBSCAN (Ester et al. 1996)) to generate *class-agnostic* prototypes $\boldsymbol{c}_p$. The SPC loss (Rao and Miao 2022) exploits the multi-scale graph features of a skeleton sequence as $\boldsymbol{v}_i$, while the MPC loss replaces it with the features of random skeleton subsequences of a sequence. By contrast, the Hi-MPC loss (Rao, Leung, and Miao 2024) constructs hierarchical skeleton representations to perform unsupervised prototype learning ($i.e.$, clustering and contrasting) at each level. However, the instability of clustering ($e.g.$, varying cluster numbers caused by over-clustering) or/and unreliability of the used *identity-agnostic* prototypes ($e.g.$, lower confidence to characterize a ground-truth identity) largely limit their practical performance.
- The graph prototype contrastive (GPC) loss in (Rao and Miao 2023) can be viewed as a *supervised* variant of the objective in Eq. (10), which adopts the ground-truth class feature centroids of skeleton graph features as the prototypes for contrastive learning. However, GPC can only perform full-relation learning of body joints without exploiting graph motifs to focus on more crucial relations from joints' structure or gait-related body components. On the other hand, although GPC combines both sequence-level and skeleton-level representation for prototype learning, it only uses their *average* spatial or temporal features, while lacking the ability to fully exploit finer-grained skeleton features such as different combinatorial patterns of spatial ($e.g.$, body-joint nodes) and temporal features ($e.g.$, skeleton graphs) for more effective skeleton pattern learning.

**Temperatures.** In our work, we adopt a generic form following the common practice (Wu et al. 2018; He et al. 2020; Chen et al. 2020; Rao and Miao 2022), $i.e.$, setting a global temperature $\tau$ for the proposed approach. By assuming a uniform feature distribution around each instance ($i.e.$, $\tau = \tau_p = \tau_j$), we encourage the model to learn representations with higher global uniformity, which could improve the quality of contrastive representation learning as theoretically and empirically proved in (Wang and Isola 2020; Gao, Yao, and Chen 2021; Rao and Miao 2022).

In the proposed approach, each ground-truth identity is represented with a unique skeleton prototype, which is generated by computing the class centroid of encoded graph representations. Our approach not only randomly masks different spatial node representations and temporal skeleton graph representations to yield their spatial-temporal combinatorial representations, but also combines both *sub-tracklet-level* and *sub-skeleton-level* skeleton prototype contrastive learning, so as to learn more identity-associated patterns and semantics from skeleton graph representations at different levels. The proposed sub-tracklet-level ($\mathcal{L}_{\mathrm{CSP}}^{str}$) and sub-skeleton-level CSP loss ($\mathcal{L}_{\mathrm{CSP}}^{ssk}$) can be formulated based on Eq. (10) as:

$$\mathcal{L}_{\mathrm{CSP}}^{str} = \frac{1}{N}\sum_{i=1}^{N} -\log \frac{\exp\left(\mathcal{M}(\boldsymbol{v}_i)\cdot \boldsymbol{c}_p/\tau_1\right)}{\sum_{j=1}^{K}\exp\left(\mathcal{M}(\boldsymbol{v}_i)\cdot \boldsymbol{c}_j/\tau_1\right)}, \tag{11}$$

$$\mathcal{L}_{\mathrm{CSP}}^{ssk} = \frac{1}{FN}\sum_{i=1}^{N}\sum_{t=1}^{F} -\log \frac{\exp\left(\hat{\mathcal{M}}(\boldsymbol{v}_i^t)\cdot \hat{\boldsymbol{c}}_p/\tau_2\right)}{\sum_{j=1}^{K}\exp\left(\hat{\mathcal{M}}(\boldsymbol{v}_i^t)\cdot \hat{\boldsymbol{c}}_j/\tau_2\right)}, \tag{12}$$

where $\boldsymbol{c}_j$, $\hat{\boldsymbol{c}}_j$ denotes the $j^{th}$ skeleton prototype and its linear projection, $i.e.$, $\hat{\boldsymbol{c}}_j = \mathcal{F}(\boldsymbol{c}_j)$, $\mathcal{M}(\cdot)$ represents the random masking and combining function in CSP (corresponding to Eq. (8) and (9) in the paper), $\mathcal{M}(\boldsymbol{v}_i)$ (equivalent to $\overline{\boldsymbol{V}}_i$ in the paper) denotes the spatial-temporal combinatorial representation (sub-tracklet representation) of the $i^{th}$ skeleton sequence, $\hat{\mathcal{M}}(\boldsymbol{v}_i^t) = \mathcal{F}'(\mathcal{M}(\boldsymbol{v}_i^t))$ ($\mathcal{M}(\boldsymbol{v}_i^t)$ is equivalent to $\hat{\boldsymbol{v}}_t^i$ in the paper, $\mathcal{F}'(\mathcal{M}(\boldsymbol{v}_i^t))$ is equivalent to $\mathcal{F}_1(\hat{\boldsymbol{v}}_t^i)$ in the paper) represents the linear projection of spatial combinatorial representation (sub-skeleton representation) of the $t^{th}$ skeleton in the $i^{th}$ sequence, $\tau_1$ and $\tau_2$ represent the global temperatures for sub-tracklet-level and sub-skeleton-level CSP learning, and $\mathcal{F}'(\cdot)$, $\mathcal{F}(\cdot)$ are linear projection heads to transform sub-skeleton-level graph representations and high-level features of skeleton prototypes into the same contrastive space. It is worth noting that the skeleton prototypes are generated from higher level ($i.e.$, sequence-level)

representations and the learnable linear projection in Eq. (12) can be viewed as integrating related graph features from both levels for contrastive learning.

Overall, the proposed CSP loss can be viewed as an enhanced generalizable skeleton prototype loss with **(1)** Motif-guided relation learning, which integrates *skeleton-specific* motifs into global and local relation learning of key joints in multi-order body structure and gait-collaborative body components; **(2)** Spatially-temporally augmented ($i.e.$, combinatorial) skeleton prototype learning, which exploits random combinatorial features of different key body-joint nodes and skeleton graphs at both sub-skeleton and sub-tracklet levels to capture more valuable identity-related patterns and semantics for person re-ID. The proposed CSP can be generalized to different scenarios and models to enhance their person re-ID performance, as demonstrated in the discussion section of our paper.

## Convergence Proof

We prove the convergence of CSP under modeling the maximum log-likelihood estimation (see Eq. (10)). Recall Eq. (2) and (3) and let

$$\begin{aligned}\ell(\theta) &= \sum_{i=1}^{N} \log p\left(\boldsymbol{x}_i;\theta\right) \\ &= \sum_{i=1}^{N} \log \sum_{j=1}^{K} p\left(\boldsymbol{x}_i,\boldsymbol{c}_j;\theta\right) \\ &= \sum_{i=1}^{N} \log \sum_{j=1}^{K} Q\left(\boldsymbol{c}_j\right) \frac{p\left(\boldsymbol{x}_i,\boldsymbol{c}_j;\theta\right)}{Q\left(\boldsymbol{c}_j\right)} \\ &\geq \sum_{i=1}^{N} \sum_{j=1}^{K} Q\left(\boldsymbol{c}_j\right) \log \frac{p\left(\boldsymbol{x}_i,\boldsymbol{c}_j;\theta\right)}{Q\left(\boldsymbol{c}_j\right)}. \end{aligned} \tag{13}$$

The above inequality holds with equality when $Q\left(\boldsymbol{c}_j\right) = p\left(\boldsymbol{c}_j;\boldsymbol{x}_i,\theta\right)$ is a constant (see Eq. (4)).

In the $t^{th}$ E-step, we have estimated the constant value $Q^{(t)}\left(\boldsymbol{c}_j\right) = p\left(\boldsymbol{c}_j;\boldsymbol{x}_i,\theta^{(t)}\right)$ based on the ground-truth class distribution. Then we have:

$$\ell\left(\theta^{(t)}\right) = \sum_{i=1}^{N}\sum_{j=1}^{K} Q^{(t)}\left(\boldsymbol{c}_j\right) \log \frac{p\left(\boldsymbol{x}_i,\boldsymbol{c}_j;\theta^{(t)}\right)}{Q^{(t)}\left(\boldsymbol{c}_j\right)}. \tag{14}$$

For the $t^{th}$ M-step, we fix $Q^{(t)}\left(\boldsymbol{c}_j\right) = p\left(\boldsymbol{c}_j;\boldsymbol{x}_i,\theta^{(t)}\right)$ and train model parameters $\theta$ to maximize Eq. (14). In this way, we can always have:

$$\begin{aligned}\ell\left(\theta^{(t+1)}\right) &\geq \sum_{i=1}^{N}\sum_{j=1}^{K} Q^{(t)}\left(\boldsymbol{c}_j\right) \log \frac{p\left(\boldsymbol{x}_i,\boldsymbol{c}_j;\theta^{(t+1)}\right)}{Q^{(t)}\left(\boldsymbol{c}_j\right)} \\ &\geq \sum_{i=1}^{N}\sum_{j=1}^{K} Q^{(t)}\left(\boldsymbol{c}_j\right) \log \frac{p\left(\boldsymbol{x}_i,\boldsymbol{c}_j;\theta^{(t)}\right)}{Q^{(t)}\left(\boldsymbol{c}_j\right)} \\ &= \ell\left(\theta^{(t)}\right). \end{aligned} \tag{15}$$

The above result that $\ell\left(\theta^{(t)}\right)$ monotonically increases with more iterations suggests the convergence of the algorithm.

The detailed convergence properties of the EM algorithm are discussed in (McLachlan and Krishnan 2007; Wu 1983). Here we only discuss the general case, and follow (Wu 1983) to make the assumptions for the EM algorithm:

- **(a)** $\Omega$ is a subset in the $r$-dimensional Euclidean space $\mathbb{R}^r$.
- **(b)** $\Omega_{\theta^{(0)}} = \left\{\theta \in \Omega : \ell(\theta) \geq \ell\left(\theta^{(0)}\right)\right\}$ is compact for any $\ell\left(\theta^{(0)}\right) > -\infty$.
- **(c)** $\ell(\cdot)$ is continuous in $\Omega$ and differentiable in the interior of $\Omega$.

Under the assumptions of **(a)**, **(b)**, and **(c)**[3], we have: **(d)** $\left\{\ell\left(\theta^{(t)}\right)\right\}_{t\geq 0}$ is bounded above for any $\theta^{(0)} \in \Omega$. As a consequence of **(d)** and the inequality (15) ($i.e.$, $\ell\left(\theta^{(t+1)}\right) \geq \ell\left(\theta^{(t)}\right)$), $\ell\left(\theta^{(t)}\right)$ converges monotonically to some $\ell^*$.

It is worth noting that there is no guarantee that $\ell^*$ is the global maximum of $\ell(\cdot)$ over $\Omega$. As reported in previous works (Hasselblad 1969; Wolfe 1970; Laird 1978; Rubin and Thayer 1982; Wu 1983), if the log-likelihood function $\ell(\cdot)$ has several (local or global) maxima and stationary points, the convergence of the EM sequence $\left\{\ell\left(\theta^{(t)}\right)\right\}$ to either type of point depends on the choice of starting point. Readers can refer to (Wu 1983; McLachlan and Krishnan 2007) for more details about different convergence cases of the EM algorithm.

The aforementioned fact may account for the performance changes ($i.e.$, small variations) of our model on the same dataset, as different random initializations of model parameters could change $\theta^{(0)}$ ($i.e.$, the starting point) hence the final convergence result. In practice, we follow (Rao et al. 2021; Rao and Miao 2023; Rao, Leung, and Miao 2024) to train the model with different random initializations on each dataset and report its average performance, which helps estimate a more stable EM convergence result with different initialized starting points.

# References


Chen, T.; Kornblith, S.; Norouzi, M.; and Hinton, G. 2020. A Simple Framework for Contrastive Learning of Visual Representations. In *International Conference on Machine Learning (ICML)*, 1597–1607.

Ester, M.; Kriegel, H.-P.; Sander, J.; Xu, X.; et al. 1996. A density-based algorithm for discovering clusters in large spatial databases with noise. In *ACM SIGKDD Conference on Knowledge Discovery and Data Mining (KDD)*, volume 96, 226–231.

Gao, T.; Yao, X.; and Chen, D. 2021. SimCSE: Simple Contrastive Learning of Sentence Embeddings. In *Proceedings of the Conference on Empirical Methods in Natural Language Processing (EMNLP)*, 6894–6910.

Hasselblad, V. 1969. Estimation of finite mixtures of distributions from the exponential family. *Journal of the American Statistical Association*, 64(328): 1459–1471.

He, K.; Fan, H.; Wu, Y.; Xie, S.; and Girshick, R. 2020. Momentum Contrast for Unsupervised Visual Representation Learning. In


[3] These assumptions can be satisfied in most practical situations. As the related proofs/discussions are out of the scope of this work, readers can refer to (Wu 1983) for more details.

*Proceedings of the IEEE/CVF Conference on Computer Vision and Pattern Recognition (CVPR)*, 9729–9738.

Laird, N. 1978. Nonparametric maximum likelihood estimation of a mixing distribution. *Journal of the American Statistical Association*, 73(364): 805–811.

Li, J.; Zhou, P.; Xiong, C.; and Hoi, S. 2021. Prototypical Contrastive Learning of Unsupervised Representations. In *International Conference on Learning Representation (ICLR)*.

McLachlan, G. J.; and Krishnan, T. 2007. *The EM algorithm and extensions*. John Wiley & Sons.

Nauta, M.; Trienes, J.; Pathak, S.; Nguyen, E.; Peters, M.; Schmitt, Y.; Schlötterer, J.; van Keulen, M.; and Seifert, C. 2022. From anecdotal evidence to quantitative evaluation methods: A systematic review on evaluating explainable AI. *arXiv preprint arXiv:2201.08164*.

Rao, H.; Leung, C.; and Miao, C. 2024. Hierarchical skeleton meta-prototype contrastive learning with hard skeleton mining for unsupervised person re-identification. *International Journal of Computer Vision*, 132(1): 238–260.

Rao, H.; and Miao, C. 2022. SimMC: Simple Masked Contrastive Learning of Skeleton Representations for Unsupervised Person Re-Identification. In *International Joint Conference on Artificial Intelligence (IJCAI)*, 1290–1297.

Rao, H.; and Miao, C. 2022. Skeleton Prototype Contrastive Learning with Multi-Level Graph Relation Modeling for Unsupervised Person Re-Identification. *arXiv preprint arXiv:2208.11814*.

Rao, H.; and Miao, C. 2023. TranSG: Transformer-Based Skeleton Graph Prototype Contrastive Learning with Structure-Trajectory Prompted Reconstruction for Person Re-Identification. In *Proceedings of the IEEE/CVF Conference on Computer Vision and Pattern Recognition (CVPR)*.

Rao, H.; Wang, S.; Hu, X.; Tan, M.; Guo, Y.; Cheng, J.; Liu, X.; and Hu, B. 2021. A self-supervised gait encoding approach with locality-awareness for 3D skeleton based person re-identification. *IEEE Transactions on Pattern Analysis and Machine Intelligence*, 44(10): 6649–6666.

Rubin, D. B.; and Thayer, D. T. 1982. EM algorithms for ML factor analysis. *Psychometrika*, 47(1): 69–76.

van den Oord, A.; Li, Y.; and Vinyals, O. 2018. Representation learning with contrastive predictive coding. *arXiv preprint arXiv:1807.03748*.

Wang, T.; and Isola, P. 2020. Understanding contrastive representation learning through alignment and uniformity on the hypersphere. In *International Conference on Machine Learning (ICML)*, 9929–9939.

Wolfe, J. H. 1970. Pattern clustering by multivariate mixture analysis. *Multivariate behavioral research*, 5(3): 329–350.

Wu, C. J. 1983. On the convergence properties of the EM algorithm. *The Annals of statistics*, 95–103.

Wu, Z.; Xiong, Y.; Yu, S. X.; and Lin, D. 2018. Unsupervised feature learning via non-parametric instance discrimination. In *Proceedings of the IEEE/CVF Conference on Computer Vision and Pattern Recognition (CVPR)*, 3733–3742.
