# Supplementary material for: Motif Guided Graph Transformer with Combinatorial Skeleton Prototype Learning for Skeleton-Based Person Re-Identification
Source: arXiv:2412.09044 source file (2025-02-02)
Supplement: Supplementary file 2 [file Appendix_I_Experiments.pdf]

# Motif Guided Graph Transformer with Combinatorial Skeleton Prototype Learning for Skeleton-Based Person Re-Identification – Appendix I Experiments

**Haocong Rao, Chunyan Miao***

College of Computing and Data Science, Nanyang Technological University (NTU), Singapore
Joint NTU-UBC Research Centre of Excellence in Active Living for the Elderly (LILY), NTU, Singapore
{haocong001,ascymiao}@ntu.edu.sg

In our supplementary materials, we provide supplementary experimental settings (see Sec. A) and results (see Sec. B) in this appendix, and offer theoretical hypotheses and analyses of our approach in Appendix II.

## A Supplementary Experimental Settings

In this section, we provide more detailed experimental settings, including dataset preprocessing strategy (Sec. A.1), probe and gallery settings (Sec. A.2), CASIA-B evaluation settings (Sec. A.3), and model implementation details (Sec. A.4).

### A.1 Dataset Preprocssing

To avoid ineffective skeleton recording, we discard the first and last 10 skeleton frames of each original skeleton sequence. For KS20, KGBD, BIWI, and IAS datasets, all skeleton sequences are normalized by subtracting the spine joint position from each joint of the same skeleton so that the skeleton is translation invariant (Zhao et al. 2019). Then, we spilt all normalized skeleton sequences in the training sets into multiple shorter skeleton sequences ($i.e.$, $\boldsymbol{X}$) with length $f$ by a step of $\frac{f}{2}$, which aims to obtain as many 3D skeleton sequences as possible to train our approach. We split all skeleton sequences in the gallery and probe sets into shorter and non-overlapping sequences with length $f$. Unless explicitly specified, the skeleton sequence $\boldsymbol{X}$ in our paper refers to those split and normalized sequences used in learning, rather than those original skeleton sequences provided by datasets. We follow the data augmentation strategy used in (Rao et al. 2021b,c) to sample more sequences for different identities in the training set, and train our approach with randomly shuffled skeleton sequences of the training set. The details of all datasets are shown in Table 1.

### A.2 Probe and Gallery Settings

We follow the commonly-used settings of probe and gallery in the literature (Rao and Miao 2022; Rao and Miao 2023; Rao, Leung, and Miao 2024): For the BIWI and IAS datasets, as different testing sets are non-overlapped and contain all pedestrians under different scenes, we evaluate our approach on each testing set by setting it as the probe while the other one is adopted as the gallery. The KGBD dataset contains different skeleton videos ($i.e.$, long skeleton sequences) of each pedestrian with varying numbers of walking rounds. Since no training/testing splits are given, we randomly choose one skeleton video of each person to split skeleton sequences and construct the probe set, and equally divide the remaining videos to build the training set and gallery set. The KS20 dataset collects skeleton data of pedestrians from five different viewpoints, including 0°, 30°, 90°, 130°, and 180°. We employ the setting of Random View Evaluation (RVE): One sequence is randomly selected from each viewpoint as the probe sequence and the remaining skeleton sequences are equally divided into gallery and training sequences. We follow the person re-ID protocols in (Liu et al. 2015) to evaluate the proposed skeleton-based approach on CASIA-B (detailed in Sec. A.3).

Table 1: Overview of datasets (K: thousand). Different testing splits are used to construct gallery sets and probe sets (see Sec. A.2). "W", "S", "A", and "B" denote BIWI-Walking, BIWI-Still, IAS-A, and IAS-B testing sets, respectively. "N", "C", and "B" represent "Normal", "Clothes", and "Bags" conditions of CASIA-B, respectively. Note: The 3D skeletons of CASIA-B are estimated from RGB videos.

| # Datasets | KGBD | BIWI | KS20 | IAS | CASIA-B |
|---|---|---|---|---|---|
| # Train IDs | 164 | 50 | 20 | 11 | 124 |
| # Train Skeletons | 188.7K | 205.8K | 36.0K | 89.0K | 706.5K |
| # Probe IDs | 164 | 28 | 20 | 11 | 62 |
| # Probe Skeletons | 94.1K | W: 4.9K<br>S: 3.2K | 3.3K | A: 7.0K<br>B: 7.8K | N: 162.1K<br>C: 54.4K<br>B: 53.9K |
| # Gallery IDs | 164 | 28 | 20 | 11 | 62 |
| # Gallery Skeletons | 188.7K | W: 4.9K<br>S: 3.2K | 3.3K | A: 7.0K<br>B: 7.8K | N: 162.1K<br>C: 54.4K<br>B: 53.9K |

### A.3 Evaluation Settings of CASIA-B

In general, 3D skeleton data in existing skeleton-based person re-ID benchmarks are collected with Kinect (Shotton et al. 2011). To evaluate the effectiveness of our approach when 3D skeleton data are directly estimated from

*Corresponding author
Copyright © 2025, Association for the Advancement of Artificial Intelligence (www.aaai.org). All rights reserved.

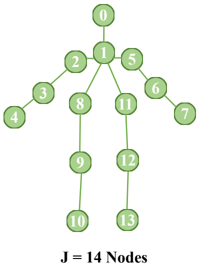


Figure 1: Node indices for graph representations of the estimated skeletons from CASIA-B dataset. Note: All 3D skeletons are extracted from RGB videos of CASIA-B by pose estimation models (Cao et al. 2019; Chen and Ramanan 2017) (see Sec. A.3). In the proposed GCM for CASIA-B, the upper limbs include 6 original joints (joint 2, 3, 4, 5, 6, and 7) while the lower limbs include 6 original joints (joint 8, 9, 10, 11, 12, and 13).

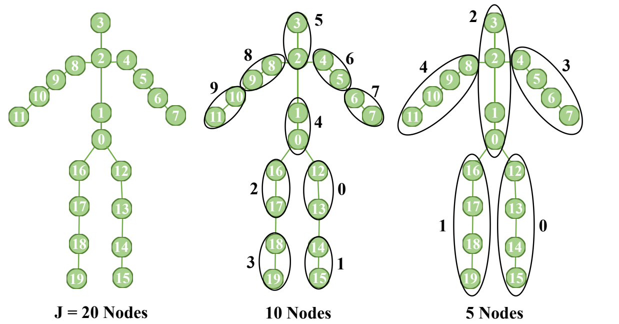


Figure 2: Node indices for joint-scale (20 nodes), part-level (10 nodes), and body-scale (5 nodes) graphs representations of skeletons from IAS, BIWI and KGBD datasets. Our approach *only* requires joint-scale graphs for training, while we evaluate its performance on different-scale graphs following (Rao et al. 2021a) in the paper. In the proposed GCM, the upper limbs include 8 original joints (joint 4, 5, 6, 7, 8, 9, 10, and 11), while the lower limbs include 8 original joints (joint 12, 13, 14, 15, 16, 17, 18, and 19). The indices correspond to the following joint names: (0) 'SpineBase', (1) 'SpineMid', (2) 'Neck', (3) 'Head', (4) 'LeftShoulder', (5) 'LeftElbow', (6) 'LeftWrist', (7) 'LeftHand', (8) 'RightShoulder', (9) 'RightElbow', (10) 'RightWrist', (11) 'RightHand', (12) 'LeftHip', (13) 'LeftKnee', (14) 'LeftAnkle', (15) 'LeftFoot', (16) 'RightHip', (17) 'RightKnee', (18) 'RightAnkle', (19) 'RightFoot'.

RGB videos rather than depth sensors such as Kinect, we use a large-scale RGB video based dataset, *CASIA-B* (Yu, Tan, and Tan 2006), which contains walking sequences of 124 individuals under 11 different views and 3 conditions—pedestrians wearing a bag ("Bags"), wearing a coat ("Clothes"), and without any coat or bag ("Normal"). We follow the evaluation setup in (Liu et al. 2015), which is frequently used in the literature: First, we randomly choose half of the individuals for training and use the rest for testing. Then, to evaluate our approach under *single-condition* and *cross-condition* settings, we divide the testing sequences by the three conditions ("Bags", "Clothes", "Normal") to construct gallery and probe sets. Specifically, for the *single-condition* setting, both gallery and probe sets use the testing sequences with the same condition (*i.e.*, gallery and probe sets are the same), and we match each sequence of the probe set with the most similar sequence from the gallery set that *excludes* the original sequence. In the *cross-condition* setting, we adopt the testing sequences under bags ("Bags") or clothes condition ("Clothes") as the probe set, and use the testing sequences under normal condition ("Normal") as the gallery set.

Following (Liao et al. 2020), we exploit pre-trained pose estimation models (Chen and Ramanan 2017; Cao et al. 2019) to extract 3D skeletons from RGB videos of CASIA-B. We first extract eighteen 2D joints from each person in videos using the *OpenPose* model (Cao et al. 2019). Then, we follow the same configuration of estimation in (Liao et al. 2020) and average the positions of "Nose", "Reye", "LEye", "Rear" and "Lear" as the position of "Head" to construct fourteen 2D joints, which are fed into the pose estimation method (Chen and Ramanan 2017) to estimate corresponding 3D body joints. Thus, the number of body-joint nodes $J$ is 14 for CASIA-B as shown in Fig. 1, and all joints in each skeleton are normalized by subtracting the neck joint.

## A.4 Implementation Details

All the important experimental details are presented in our paper. The numbers of body joints are $J = 20$ (IAS, BIWI, KGBD) and $J = 25$ (KS20) in the original datasets. We construct corresponding skeleton graphs with the same number of body-joint nodes in the original skeletons. To verify the generality of our approach when applied to different-scale skeleton graphs, we follow (Rao et al. 2021a) to construct another two scales, namely part-scale (10 nodes) and body-scale (5 nodes), by merging joints within different body partitions. The original skeleton graphs, part-scale graphs, and body-scale graphs as shown in Fig. 2 and 3. We also show the upper and lower limbs' joints used for GCM construction in Fig. 1, 2, and 3. The skeleton sequence length $f$ on four skeleton-based datasets (IAS, KS20, BIWI, KGBD) is set to 6 following (Rao and Miao 2022; Rao and Miao 2023; Rao, Leung, and Miao 2024) for a fair comparison with existing methods. As to CASIA-B, it is a large-scale dataset with roughly estimated skeleton data from RGB frames, which is intrinsically different from the previous datasets. We adopt a longer sequence length $f = 40$. The embedding size of each node representation is $D = 128$ for all datasets. We follow (Rao and Miao 2023) to set $K = 10$ for the positional encoding, and empirically employ 2 MGT layers with $H = 8$ relation heads and $D_{\mathrm{k}} = 16$ for each layer, as these settings achieve the best average performance on different datasets. We follow (Dwivedi et al. 2020; Dwivedi and Bresson 2021) to randomly flip the sign of the eigenvectors during training to improve the model stability on small datasets (IAS, KS20, BIWI). For part-scale (10 nodes) and body-scale (5 nodes) skeleton graphs compared with SM-SGE, we correspondingly set $K = 9$ and $K = 4$ for the positional en-

Table 2: Full results for ablation study on different components: Graph transformer (GT), hierarchical structural motifs (HSM), gait collaborative motifs (GCM), and combinatorial skeleton prototype learning (CSP). ✓indicates using the component.

| ID | GT | HSM | GCM | CSP | BIWI-S | | BIWI-W | | KS20 | | KGBD | | IAS-A | | IAS-B | |
|---|---|---|---|---|---|---|---|---|---|---|---|---|---|---|---|---|
| | | | | | $R_1$ | mAP | $R_1$ | mAP | $R_1$ | mAP | $R_1$ | mAP | $R_1$ | mAP | $R_1$ | mAP |
| **1** | | | | | 38.1 | 11.3 | 21.2 | 18.3 | 64.8 | 20.5 | 53.0 | 11.0 | 39.2 | 17.8 | 40.7 | 21.5 |
| **2** | ✓ | | | | 66.6 | 26.7 | 31.2 | 25.5 | 71.3 | 42.5 | 57.0 | 18.1 | 48.0 | 31.8 | 56.1 | 37.9 |
| **3** | ✓ | ✓ | | | 69.0 | 29.1 | 33.0 | 27.1 | 74.5 | 48.4 | 59.3 | 24.1 | 49.3 | 33.7 | 58.2 | 43.2 |
| **4** | ✓ | | ✓ | | 69.4 | 29.6 | 34.0 | 28.2 | 74.4 | 48.9 | 60.2 | 24.0 | 50.4 | 34.2 | 59.5 | 44.8 |
| **5** | ✓ | ✓ | ✓ | | 70.8 | 31.4 | 34.5 | 29.4 | 75.2 | 50.1 | 60.9 | 25.8 | 50.8 | 34.9 | 60.6 | 45.2 |
| **6** | ✓ | ✓ | ✓ | ✓ | 72.0 | 32.1 | 36.0 | 30.5 | 76.0 | 50.8 | 62.0 | 26.1 | 51.9 | 35.8 | 61.5 | 45.5 |

Table 3: The number of network parameters (million (M)) and computational complexity (giga floating-point operations (GFLOPs)) of deep learning based methods. ♠ denotes skeleton graph based methods, † indicates using hand-crafted descriptors, and ‡ refers to sequence representation learning models. Note: Both numbers of parameters and GFLOPs in the training of neural networks are counted by the Tensorflow platform (Abadi et al. 2016). Extra matrix computation is required for the clustering in SimMC and Hi-MPC (see Sec. B.1).

| Methods | # Params | GFLOPs |
|---|---|---|
| PoseGait† (Liao et al. 2020) | 8.93M | 121.60 |
| MG-SCR♠ (Rao et al. 2021c) | 0.35M | 6.60 |
| AGE‡ (Rao et al. 2020) | 7.15M | 37.37 |
| SGELA‡ (Rao et al. 2021b) | 8.47M | 7.47 |
| SM-SGE♠ (Rao et al. 2021a) | 5.58M | 22.61 |
| Hi-MPC‡ (Rao, Leung, and Miao 2024) | 3.32M | 3.37 |
| MoCos♠ (Ours) | 0.40M | 20.22 |

coding. For main experiments, we empirically set spatial and temporal masking probabilities for different datasets: $p_s = 0.25$, $p_t = 0.25$ for IAS-B, BIWI, KS20, $p_s = 0.5$, $p_t = 0.1$ for IAS-A, and $p_s = 0.5$, $p_t = 0.25$ for KGBD. We use fusion coefficient $\lambda = 0.9$ for BIWI-W, KGBD, KS20, $\lambda = 0.25$ for BIWI-S, $\lambda = 0.75$ for IAS-A and IAS-B. For the discussed experiments with RGB-estmiated skeletons, we empirically set $\alpha = 1.0$ as it can achieve better performance. It should be noted that the models trained with RGB-estimated skeletons possess some performance variations, possibly due to the noise in roughly-estimated skeletons. We thus select the models with slightly better overall performance ($i.e.$, higher mAP instead of higher Rank-1 accuracy) for the discussion in the paper. We will provide a systematic analysis for the model initializations and performance variations in our future works. We empirically set $\tau_1 = 0.1$ and $\tau_2 = 10$ for contrastive learning in subtracklet-level and sub-skeleton-level CSP. An Adam optimizer with the learning rate of of $3.5 \times 10^{-4}$ is used for the model optimization, and we set batch size to 256 for all datasets. To avoid over-fitting and achieve better generalization performance, we adopt Early Stopping (Prechelt 1998) with a patience of 150 epochs ($i.e.$, stop the training of model after no improvement in 150 continuous epochs). The experiments are repeated for multiple time with random model parameter initialization for training, and we report the average performance for a fair comparison with existing methods. Our models are trained and tested on 1x NVIDIA Tesla V100 (32GB) and P100 (16GB) GPUs with the 2x Intel(R) Xeon(R) Gold 6148 CPU @2.40GHz. Multiple ex-

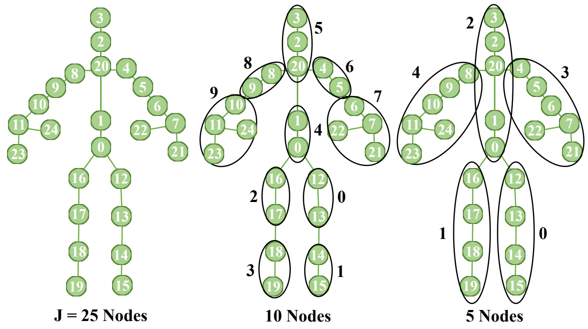


Figure 3: Node indices for joint-scale (25 nodes), part-level (10 nodes), and body-scale (5 nodes) graphs representations of skeletons from KS20 dataset. Our approach *only* requires joint-scale graphs for training, while we evaluate its performance on different-scale graphs following (Rao et al. 2021a) in the paper. In the proposed GCM, the upper limbs include 12 original joints (joint 4, 5, 6, 7, 21, 22, 8, 9, 10, 11, 23, and 24) while the lower limbs include 8 original joints (joint 12, 13, 14, 15, 16, 17, 18, and 19). The indices correspond to the following joint names: (0) 'SpineBase', (1) 'SpineMid', (2) 'Neck', (3) 'Head', (4) 'LeftShoulder', (5) 'LeftElbow', (6) 'LeftWrist', (7) 'LeftHand', (8) 'RightShoulder', (9) 'RightElbow', (10) 'RightWrist', (11) 'RightHand', (12) 'LeftHip', (13) 'LeftKnee', (14) 'LeftAnkle', (15) 'LeftFoot', (16) 'RightHip', (17) 'RightKnee', (18) 'RightAnkle', (19) 'RightFoot', (20) 'SpineShoulder', (21) 'LeftHandTip', (22) 'LeftThumb', (23) 'RightHandTip', (24) 'RightThumb'.

periments with the same or different configurations can be parallelly conducted on our device. Readers can access our source code[1] for more details of the used libraries and frameworks.

For all methods compared in our experiments, we select optimal model parameters for training, and use their predefined skeleton descriptors or pre-trained skeleton representations for person re-ID. It is worth noting that our reimplementations of some existing models get performance with slight variations, and the results are basically the same as the original papers under different random model initializations. For a fair comparison, we follow (Rao et al. 2021b; Rao and Miao 2022; Rao and Miao 2023) to report the average performance of all methods. Note that our ap-

[1]Our anonymized code and data are publicly available at https://github.com/Anonymous-4136/MoCos

Table 4: Performance of our approach on different datasets when setting different fusion coefficients $\lambda$ to fuse sub-tracklet-level ($\mathcal{L}_{\text{CSP}}^{str}$) and sub-skeleton-level combinatorial prototype learning ($\mathcal{L}_{\text{CSP}}^{ssk}$).

| $\lambda$ | KS20 | | KGBD | | IAS-A | | IAS-B | | BIWI-W | | BIWI-S | |
|---|---|---|---|---|---|---|---|---|---|---|---|---|
| | **mAP** | **$R_1$** | **mAP** | **$R_1$** | **mAP** | **$R_1$** | **mAP** | **$R_1$** | **mAP** | **$R_1$** | **mAP** | **$R_1$** |
| **0.10** | 48.1 | 75.2 | 15.3 | 56.1 | 33.4 | 49.4 | 45.2 | 58.2 | 27.7 | 33.3 | 30.6 | 70.8 |
| **0.25** | 49.1 | 75.3 | 16.4 | 56.7 | 32.0 | 49.2 | 44.7 | 57.9 | 28.2 | 33.7 | 32.1 | 72.0 |
| **0.50** | 48.6 | 74.4 | 23.5 | 58.4 | 34.0 | 50.0 | 45.3 | 61.2 | 29.6 | 34.6 | 31.2 | 70.9 |
| **0.75** | 50.1 | 75.6 | 26.0 | 61.5 | 35.8 | 51.9 | 45.5 | 61.5 | 30.1 | 35.6 | 31.8 | 71.3 |
| **0.90** | 50.8 | 76.0 | 26.1 | 62.0 | 34.3 | 49.1 | 45.4 | 60.9 | 30.5 | 36.0 | 29.7 | 70.9 |

Table 5: Performance of our approach on different datasets when setting different probability $p_s$ for randomly masking spatial skeleton features ($i.e.$, body-joint nodes) in the proposed CSP.

| $p_s$ | KS20 | | KGBD | | IAS-A | | IAS-B | | BIWI-W | | BIWI-S | |
|---|---|---|---|---|---|---|---|---|---|---|---|---|
| | **mAP** | **$R_1$** | **mAP** | **$R_1$** | **mAP** | **$R_1$** | **mAP** | **$R_1$** | **mAP** | **$R_1$** | **mAP** | **$R_1$** |
| **0.00** | 50.4 | 74.9 | 26.0 | 60.5 | 34.0 | 50.3 | 43.3 | 60.3 | 29.7 | 35.7 | 31.5 | 71.1 |
| **0.25** | 50.8 | 76.0 | 25.9 | 61.2 | 35.7 | 51.6 | 45.5 | 61.5 | 30.5 | 36.0 | 32.1 | 72.0 |
| **0.50** | 50.3 | 75.6 | 26.1 | 62.0 | 35.8 | 51.9 | 45.7 | 59.3 | 29.1 | 35.9 | 31.5 | 71.4 |
| **0.75** | 49.6 | 73.4 | 23.6 | 58.8 | 35.5 | 51.4 | 42.5 | 53.6 | 29.0 | 35.6 | 26.2 | 58.5 |

proach does not use any post-processing technique, $e.g.$, re-ranking (Zhong et al. 2017) or multi-query fusion (Zheng et al. 2015) in the training or testing stage. To perform person re-ID, we exploit the approach to encode each original skeleton sequence of the probe set $\Phi_{\mathcal{P}}$ into corresponding sequence-level graph representations, $\{\boldsymbol{X}_i^{\mathcal{P}}\}_{i=1}^{n_2}$, and match it with representations, $\{\boldsymbol{X}_i^{\mathcal{G}}\}_{i=1}^{n_3}$, of the same identity in the gallery set $\Phi_{\mathcal{G}}$ using Euclidean distance. In the ablation study, we use the concatenation of raw skeleton sequences ($i.e.$, normalized 3D coordinates of body joints) to perform direct prototype learning (DP) as the baseline. For the configuration of skeleton graph transformer (GT) with graph prototype learning, we adopt the same setting used in (Rao and Miao 2023).

For the discussed experiments ("Transfer to Unsupervised Paradigms") with the configuration "+ MoCos", we employ the first component of MoCos, $i.e.$, MGT, to encode skeletal relations and features, then apply the second component of MoCos, $i.e.$, CSP, to generate spatial-temporal combinatorial skeleton representations for prototype learning of SimMC and SPC-MGR. For "SimMC + MoCos", since the MPC component in SimMC possesses the similar function of temporal skeleton masking ($i.e.$, generating temporal combinatorial skeleton features with masks), we slightly modify MoCos to randomly mask the body-joint node representations to perform CSP. We empirically adopt $p_s = 0.25$ for KS20 and $p_s = 0.1$ for other datasets. The numbers of MGT layers are empirically set to 3, 1, 1, 2 to train the new model on IAS, BIWI, KGBD, KS20 datasets respectively. For KGBD, we set the temperature $\tau = 0.005$. For "SPC-MGR + MoCos", we empirically set $p_s = 0.1$, $p_s = 0.5$ and apply CSP to all different skeleton levels used in SPC-MGR. It is worth noting that we utilize the full-level collaborative relation layer in SPC-MGR to perform the full-relation learning function in MGT, and integrate HSM and GCM into them. Since this compatible relation learning way is not a standard form of MoCos and may not fully reflect its actual effectiveness, we only use its performance as a reference for comparison with other unsupervised paradigms applied MoCos. All other parameter settings are kept the same with (Rao and Miao 2022; Rao and Miao 2022). For the "Feature and Relation Visualization" part, the mean relational values are computed by averaging matrices over all relation heads and all skeleton graphs in the same sequence. This aims to show the relation diversity and magnitude of all heads (motif guided or non-motif guided heads) in MoCos to compare with only using full-relation learning without motifs in TranSG (Rao and Miao 2023).

# B Supplementary Results

In this section, we provide full experimental results for ablation study (Table 2), model efficiency (Sec. B.1), effects of hyper-parameters (Sec. B.2, Table 4-11), multi-shot performance with different sequence lengths $f$ (Sec. B.3), visualization of body-component relations (Sec. B.4), training metrics (different losses) (Sec. B.5), and confusion matrices (Sec. B.6).

## B.1 Model Efficiency

We report the model efficiency in terms of model size, $i.e.$, number of network parameters, and computational complexity for existing deep learning based methods. For the model that possesses varying sizes and complexities on different datasets due to the changes of input data, we report the largest case. As shown in Table 3, the proposed approach possesses smaller model size than many existing skeleton-based person re-ID methods (PoseGait (Liao et al. 2020), AGE (Rao et al. 2020), SGELA (Rao et al. 2021b), SM-SGE (Rao et al. 2021a), Hi-MPC (Rao, Leung, and Miao 2024)). The number of GFLOPs in Table 3 refers to computational complexity in the training of neural networks, which is the whole[2]/main computational complexity for deep learning methods. It should be noted that the unsupervised prototype contrastive learning (SimMC (Rao and Miao 2022), Hi-MPC (Rao, Leung, and Miao 2024)) requires extra matrix computation ($e.g.$, vector similarity query) for

[2]For representation learning methods without other learning processes ($e.g.$, clustering), the whole computational complexity of the model can be equivalent to the computational complexity of the used neural networks.

Table 6: Performance of our approach on different datasets when setting different probability $p_t$ for randomly masking temporal skeleton features ($i.e.$, skeleton graph representations) in the proposed CSP.

| $p_t$ | KS20 | | KGBD | | IAS-A | | IAS-B | | BIWI-W | | BIWI-S | |
|---|---|---|---|---|---|---|---|---|---|---|---|---|
| | **mAP** | **R$_1$** | **mAP** | **R$_1$** | **mAP** | **R$_1$** | **mAP** | **R$_1$** | **mAP** | **R$_1$** | **mAP** | **R$_1$** |
| **0.00** | 49.9 | 73.4 | 26.0 | 60.5 | 35.6 | 50.8 | 46.0 | 60.4 | 29.9 | 34.1 | 30.8 | 70.4 |
| **0.10** | 50.0 | 75.0 | 26.3 | 61.1 | 35.8 | 51.9 | 44.5 | 60.9 | 30.2 | 34.9 | 31.5 | 71.8 |
| **0.25** | 50.8 | 76.0 | 26.1 | 62.0 | 32.9 | 48.0 | 45.5 | 61.5 | 30.5 | 36.0 | 32.1 | 72.0 |
| **0.50** | 50.5 | 76.2 | 24.7 | 59.5 | 33.0 | 49.2 | 45.9 | 57.3 | 30.5 | 34.4 | 31.9 | 72.4 |
| **0.75** | 50.0 | 75.7 | 25.0 | 59.2 | 32.8 | 49.3 | 45.1 | 55.6 | 30.9 | 35.0 | 32.0 | 72.2 |

Table 7: Performance of our approach on different datasets when setting different numbers of relation heads per MGT layer.

| $H$ | KS20 | | KGBD | | IAS-A | | IAS-B | | BIWI-W | | BIWI-S | |
|---|---|---|---|---|---|---|---|---|---|---|---|---|
| | **mAP** | **R$_1$** | **mAP** | **R$_1$** | **mAP** | **R$_1$** | **mAP** | **R$_1$** | **mAP** | **R$_1$** | **mAP** | **R$_1$** |
| **8** | 50.8 | 76.0 | 26.1 | 62.0 | 35.8 | 51.9 | 45.5 | 61.5 | 30.5 | 36.0 | 32.1 | 72.0 |
| **16** | 51.5 | 76.6 | 26.8 | 62.3 | 36.1 | 51.2 | 44.9 | 61.7 | 30.8 | 35.7 | 33.2 | 70.2 |
| **32** | 51.0 | 75.8 | 26.3 | 62.2 | 36.5 | 52.3 | 42.7 | 61.4 | 31.3 | 35.6 | 30.1 | 65.6 |

the clustering process , which is usually time-consuming and computationally expensive as it may require both CPU and GPU ($e.g.$, using Faiss library (Johnson, Douze, and Jégou 2019)). In contrast, our approach exploits ground-truth identities to generate graph prototypes, which can not only improve the prototype reliability but also achieve significantly faster training without requiring clustering. On the other hand, compared with directly using full-relation learning in TranSG (Rao and Miao 2023), our approach that incorporates motif-guided relation learning and combinatorial skeleton prototype learning possesses highly similar parameter size but can achieve significantly higher performance on different scenarios, as demonstrated in our paper.

## B.2 Effects of Different Hyper-Parameters

**Effects of different fusion coefficients $\lambda$:** As shown in Table 4, our approach achieves better performance in most datasets when setting a relatively higher value of $\lambda$ ($i.e.$, 0.75-0.9) to fuse sub-tracklet-level and sub-skeleton-level combinatorial skeleton prototype learning (CSP). This could suggest the higher contribution and efficiency of sub-tracklet-level CSP, possibly because it can help the model directly learn more discriminative skeleton representations at the (sub)sequence level instead of (sub)skeleton level, better matching the target of our task to exploit skeleton sequence representations to perform person re-ID. Compared with mainly using sub-skeleton-level CSP ($i.e.$, $\lambda = 0.10$), the higher performance when setting $\lambda = 0.5$ can demonstrate the compatibility of both sub-tracklet-level and sub-skeleton-level CSP to facilitate each other to learn more effective skeleton graph representations. Interestingly, we observe that an appropriate fusion on some datasets such as BIWI-S is crucial to obtain better results. As the skeleton data of different domains ($e.g.$, datasets) are collected under different conditions, the context of skeleton structure (corresponding to spatial masking) or motion (corresponding to temporal masking) may have different contributions on the skeleton semantics learning (also consistent with the analyses in (Rao and Miao 2023)), thus $\lambda$ could be further selected to facilitate the model training.

**Effects of different probabilities $p_s$ and $p_t$ for random spatial and temporal masking:** Compared with the model without using spatial or temporal combinatorial CSP ($i.e.$, $p_s = 0.00$ or $p_t = 0.00$), using a moderate random probability ($e.g.$, 0.25-0.5) to generate diverse spatial-temporal combinatorial skeleton features enables the model to achieve the best performance in average on different datasets, as shown in Table 5 and Table 6. This further demonstrates the effectiveness of the proposed CSP with random probabilistic masking, as analyzed in our paper. However, using a very high value of masking probability ($e.g.$, $p_s = 0.75$) could slightly reduce the overall performance of our model on most datasets, which implies that using less informative combinatorial skeleton representations such as very few skeleton joints or frames might add the difficulty of learning more discriminative representations and result in lower effectiveness of CSP. In our work, the random masking probabilities $p_s$ and $p_t$ are empirically selected for better model learning on different datasets.

**Effects of different numbers of relation heads and MGT layers:** As shown in Table 8, setting 2 MGT layers with 8 relation heads (including 5 motif guided relation heads and 3 FR heads) per layer enables our model to obtain the best performance on different datasets. The results in Table 7 also suggest that adding more relation heads can further improve the model performance, as they facilitate the model to jointly attend to more valuable relational features from different feature subspaces. However, employing too many numbers of relation heads ($e.g.$, $H = 32$) slightly reduces the performance as it might capture more similar or redundant information in the heads and possibly result in the degradation of relation learning. Adopting more than two MGT layers cannot benefit the model learning with similar performance on KS20, IAS-A, and IAS-B, while the models trained on KGBD and BIWI are more sensitive to the layer variation. It is possibly because adding layers largely expands the model scale to cause more redundant parameters and features under the same training data size, while the cascade relational learning within more layers may induce more loss of explicit and effective relational information. In our paper, we empirically select $H = 8$ heads and two MGT layers to achieve a better trade-off between computational cost and performance.

**Effects of other parameters:** As shown in Table 9 and

Table 8: Performance of our approach on different datasets when setting different numbers of Motif guided skeleton Graph Transformer (MGT) layers.

| Layers | KS20 | | KGBD | | IAS-A | | IAS-B | | BIWI-W | | BIWI-S | |
|---|---|---|---|---|---|---|---|---|---|---|---|---|
| | mAP | $R_1$ | mAP | $R_1$ | mAP | $R_1$ | mAP | $R_1$ | mAP | $R_1$ | mAP | $R_1$ |
| **1** | 44.7 | 70.7 | 20.1 | 59.1 | 34.7 | 51.1 | 43.0 | 57.2 | 28.6 | 35.4 | 26.4 | 68.6 |
| **2** | 50.8 | 76.0 | 26.1 | 62.0 | 35.8 | 51.9 | 45.5 | 61.5 | 30.5 | 36.0 | 32.1 | 72.0 |
| **3** | 49.3 | 73.1 | 21.7 | 57.0 | 35.0 | 51.6 | 44.8 | 59.9 | 30.2 | 36.2 | 25.6 | 66.4 |
| **4** | 41.1 | 72.3 | 19.8 | 56.6 | 33.4 | 51.5 | 39.0 | 57.3 | 22.7 | 29.4 | 22.9 | 65.6 |

Table 9: Performance of our approach on different datasets when setting different temperature $\tau_1$.

| $\tau_1$ | KS20 | | KGBD | | IAS-A | | IAS-B | | BIWI-W | | BIWI-S | |
|---|---|---|---|---|---|---|---|---|---|---|---|---|
| | mAP | $R_1$ | mAP | $R_1$ | mAP | $R_1$ | mAP | $R_1$ | mAP | $R_1$ | mAP | $R_1$ |
| **0.01** | 48.7 | 74.8 | 20.2 | 61.1 | 33.3 | 49.7 | 44.6 | 59.5 | 30.3 | 35.0 | 31.2 | 71.7 |
| **0.1** | 50.8 | 76.0 | 26.1 | 62.0 | 35.8 | 51.9 | 45.5 | 61.5 | 30.5 | 36.0 | 32.1 | 72.0 |
| **1.0** | 47.3 | 73.6 | 16.8 | 57.3 | 35.0 | 51.3 | 43.8 | 61.3 | 29.8 | 31.6 | 29.6 | 65.6 |
| **10** | 43.2 | 72.5 | 14.9 | 55.1 | 35.1 | 52.1 | 44.5 | 59.7 | 27.4 | 32.9 | 26.5 | 57.2 |

Table 10, our approach is not very sensitive to changes of some parameters such as temperatures $\tau_1$ and $\tau_2$ on most datasets (KS20, IAS-A, IAS-B, BIWI-W). It is observed that $\tau_2$ is a more influential factor than $\tau_1$ on different datasets, while setting too small value of $\tau_2$ could significantly reduce the performance especially mAP in most cases. The results in 10 show that MoCos achieves higher performance when setting a relatively higher value for the temperature $\tau_2$, which also improves the training stability ($i.e.$, smaller loss fluctuation) of our model on different datasets. Although setting different $\tau_1$ value may obtain similar results, we observe that their scales could influence the training stability ($i.e.$, setting too small or too large values induces more evident performance variations). We therefore choose a moderate value for the temperature $\tau_1$. In our experiments, the temperatures are empirically set to $\tau_1 = 0.1$ and $\tau_2 = 10$, and they could be further tuned for better performance.

## B.3 Multi-Shot Performance with Different Lengths $f$

We evaluate the multi-shot performance of our approach with different settings of sequence lengths $f$ ($i.e.$, $f$-shot person re-ID). Since skeleton sequences contain more pattern features as $f$ increases, our approach is capable of learning more effective skeleton graph representations to achieve larger performance improvement in most cases as shown in 11. Nevertheless, it is interesting to note that using shorter sequences sometimes performs better than longer sequences on small datasets such as IAS-B and BIWI-S, implying that a larger size of available training sequences under smaller $f$ settings could help learn better representations on those datasets. It should be noted that in our paper, we evaluate all compared methods under the same sequence length ($f = 6$) following the literature (Rao and Miao 2022; Rao and Miao 2023).

## B.4 Visualization of Body Relations

As shown in Fig. 9-16, we visualize relations learned from three different heads (including the $1^{th}$ head corresponding to HSM $\mathcal{A}^1$, the $4^{th}$ head corresponding to GCM $\mathcal{B}^1$, the $8^{th}$ head corresponding to full relations without motifs) for the same skeleton sequence in different datasets. Note that there are totally $H = 8$ learned relation matrices in our approach and here we only visualize 3 of them. Since each head computes $f$ relation matrices corresponding to $f$ skeleton graphs in a sequence, we average them into a matrix to show the mean relations of body-joint nodes. We can observe that different heads can capture different correlations between different nodes, and they can individually focus on patterns of the same body part correlated with other parts. For example, the $4^{th}$ head trained on KGBD focuses on salient relations between nodes 2-4 and nodes 0-8 (see Fig. 13 (b)), while the $8^{th}$ head not only assigns weights to these parts but also pays diverse attention to patterns between nodes 2-4 and other body components ($i.e.$, nodes 10-13 and 16-19 (see Fig. 13 (c)). These results demonstrate that different motif-guided and full-relation heads in our approach can capture different body and motion relations of nodes from different representation subspaces to facilitate learning a better skeleton graph representation.

## B.5 Visualization of Training Process

We visualize the total training loss $\mathcal{L}_{\text{CSP}}$ in Fig. 4, and the results show that our model learning converges in the first 100 to 150 optimization epochs for relatively small datasets (KS20, IAS, BIWI) and about 300 epochs for large datasets (KGBD). Meanwhile, the sub-skeleton level CSP loss $\mathcal{L}_{\text{CSP}}^{ssk}$ and sub-tracklet level loss curves $\mathcal{L}_{\text{CSP}}^{str}$ present similar learning tendency and effects with $\mathcal{L}_{\text{CSP}}$, as individually presented in Fig. 5 and 6. This validates our intuition that the sub-skeleton level CSP and the sub-tracklet level CSP in our model are compatible and they can be combined to facilitate the model training. Notably, it is observed that the sub-tracklet level loss $\mathcal{L}_{\text{CSP}}^{str}$ converges more slowly than the $\mathcal{L}_{\text{CSP}}^{ssk}$ on datasets with larger number of identities (KGBD) or more views (KS20). This may implies that datasets containing more skeleton samples or scenarios could benefit more from the sub-tracklet-level combinatorial skeleton prototype learning, as it can simultaneously generate more diverse spatial and temporal combinatorial skeleton features ($i.e.$, more random samples of combining different body-joint nodes and skeleton graphs) to expand the training space and enhance the model learning.

To provide a further analysis of the learned skeleton rep-

Table 10: Performance of our approach on different datasets when setting different temperature $\tau_2$.

| $\tau_2$ | KS20 | | KGBD | | IAS-A | | IAS-B | | BIWI-W | | BIWI-S | |
|---|---|---|---|---|---|---|---|---|---|---|---|---|
| | **mAP** | **$R_1$** | **mAP** | **$R_1$** | **mAP** | **$R_1$** | **mAP** | **$R_1$** | **mAP** | **$R_1$** | **mAP** | **$R_1$** |
| **0.01** | 35.4 | 71.3 | 15.2 | 56.9 | 35.0 | 51.7 | 37.6 | 57.1 | 23.9 | 23.7 | 23.9 | 66.8 |
| **0.1** | 45.8 | 72.5 | 16.5 | 56.6 | 33.1 | 50.5 | 39.8 | 60.2 | 22.7 | 24.9 | 23.9 | 69.5 |
| **1.0** | 48.9 | 75.0 | 16.7 | 59.6 | 35.1 | 50.6 | 45.0 | 59.8 | 30.3 | 31.9 | 30.2 | 70.4 |
| **10** | 50.8 | 76.0 | 26.1 | 62.0 | 35.8 | 51.9 | 45.5 | 61.5 | 30.5 | 36.0 | 32.1 | 72.0 |

Table 11: Performance of our approach on different datasets when employing different sequence length $f$.

| $f$ | KS20 | | KGBD | | IAS-A | | IAS-B | | BIWI-W | | BIWI-S | |
|---|---|---|---|---|---|---|---|---|---|---|---|---|
| | **mAP** | **$R_1$** | **mAP** | **$R_1$** | **mAP** | **$R_1$** | **mAP** | **$R_1$** | **mAP** | **$R_1$** | **mAP** | **$R_1$** |
| **4** | 50.7 | 76.2 | 26.2 | 61.7 | 33.5 | 50.8 | 44.3 | 58.2 | 29.6 | 34.1 | 33.3 | 71.2 |
| **6** | 50.8 | 76.0 | 26.1 | 62.0 | 35.8 | 51.9 | 45.5 | 61.5 | 30.5 | 36.0 | 32.1 | 72.0 |
| **8** | 53.9 | 77.0 | 27.7 | 61.9 | 43.9 | 53.9 | 49.3 | 62.5 | 38.3 | 37.1 | 38.4 | 76.0 |
| **10** | 56.9 | 80.9 | 26.5 | 62.0 | 42.7 | 55.6 | 49.1 | 59.7 | 40.6 | 41.0 | 39.7 | 74.2 |

resentations, we follow (Rao and Miao 2022; Rao and Miao 2023) to estimate the *mean intra-class tightness (mACT)* and *mean inter-class looseness (mRCL)* of the learned skeleton graph representations $w.r.t.$ the ground-truth classes. The mACT and mRCL can serve as effective evaluation metrics of the contrastive representation learning and identity-associated semantics learning[3]. As shown in Fig. 7 and 8, the training of our approach progressively improves both mACT and mRCL of the learned skeleton graph representations on different datasets, which demonstrates that the proposed MoCos is able to capture effective class-related semantics ($e.g.$, inter-class differences) to learn more discriminative skeleton representations for person re-ID.

### B.6 Confusion Matrix Visualization

As shown in Fig. 17, we visualize the confusion matrices of our approach when performing person re-ID with the Rank-1 matching ($i.e.$, predicting the identity of each probe sequence using the Rank-1 gallery sequence that has the smallest Euclidean distance) on all testing sets (probe sets). Fig. 17 (a)-(f) show that each confusion matrix possesses an evident alignment between the predicted identities and the ground-truth identities on the diagonal line. This suggests that skeleton sequences in most classes can be correctly matched between the probe set and gallery set in each dataset. Moreover, it can be seen that the ratios of classes with high accuracy ($i.e.$, ratios of red grids on the diagonal line) in KS20, BIWI-S, and KGBD are larger than that in IAS-A, IAS-B, and BIWI-W. The larger numbers of white and red grids diffused *around* the diagonal lines, which represent the higher proportions of false matches, on the matrices of IAS-A (see Fig. 17 (e)) and BIWI-W (see Fig. 17 (d)) imply that our model tends to confuse skeleton sequences of more different identities on these datasets. These results are consistent with the performance results shown in the paper.

[3]According to the criterion in (Rao and Miao 2022), a good model should satisfy: The same-class representations are gathered closer (higher mACT) while different-class representations possess larger distances (higher mRCL).

## References


Abadi, M.; Barham, P.; Chen, J.; Chen, Z.; Davis, A.; Dean, J.; Devin, M.; Ghemawat, S.; Irving, G.; Isard, M.; et al. 2016. Tensorflow: A system for large-scale machine learning. In *12th USENIX Symposium on Operating Systems Design and Implementation OSDI 16)*, 265–283.

Cao, Z.; Hidalgo, G.; Simon, T.; Wei, S.-E.; and Sheikh, Y. 2019. OpenPose: Realtime multi-person 2D pose estimation using Part Affinity Fields. *IEEE Transactions on Pattern Analysis and Machine Intelligence*, 43(1): 172–186.

Chen, C.-H.; and Ramanan, D. 2017. 3D human pose estimation= 2D pose estimation+ matching. In *Proceedings of the IEEE/CVF Conference on Computer Vision and Pattern Recognition (CVPR)*, 7035–7043.

Dwivedi, V. P.; and Bresson, X. 2021. A generalization of transformer networks to graphs. In *AAAI Conference on Artificial Intelligence (AAAI) Workshop*.

Dwivedi, V. P.; Joshi, C. K.; Laurent, T.; Bengio, Y.; and Bresson, X. 2020. Benchmarking graph neural networks. *arXiv preprint arXiv:2003.00982*.

Johnson, J.; Douze, M.; and Jégou, H. 2019. Billion-scale similarity search with gpus. *IEEE Transactions on Big Data*, 535–547.

Liao, R.; Yu, S.; An, W.; and Huang, Y. 2020. A model-based gait recognition method with body pose and human prior knowledge. *Pattern Recognition*, 98: 107069.

Liu, Z.; Zhang, Z.; Wu, Q.; and Wang, Y. 2015. Enhancing person re-identification by integrating gait biometric. *Neurocomputing*, 168: 1144–1156.

Prechelt, L. 1998. Early Stopping-But When? In *Advances in Neural Information Processing Systems (NeurIPS) Workshop*, 55–69.

Rao, H.; Hu, X.; Cheng, J.; and Hu, B. 2021a. SM-SGE: A Self-Supervised Multi-Scale Skeleton Graph Encoding Framework for Person Re-Identification. In *Proceedings of the 29th ACM International Conference on Multimedia*, 1812–1820.

Rao, H.; Leung, C.; and Miao, C. 2024. Hierarchical skeleton meta-prototype contrastive learning with hard skeleton mining for unsupervised person re-identification. *International Journal of Computer Vision*, 132(1): 238–260.

Rao, H.; and Miao, C. 2022. SimMC: Simple Masked Contrastive Learning of Skeleton Representations for Unsupervised Person Re-Identification. In *International Joint Conference on Artificial Intelligence (IJCAI)*, 1290–1297.

Rao, H.; and Miao, C. 2022. Skeleton Prototype Contrastive Learning with Multi-Level Graph Relation Modeling for Unsupervised Person Re-Identification. *arXiv preprint arXiv:2208.11814*.

Rao, H.; and Miao, C. 2023. TranSG: Transformer-Based Skeleton Graph Prototype Contrastive Learning with Structure-Trajectory

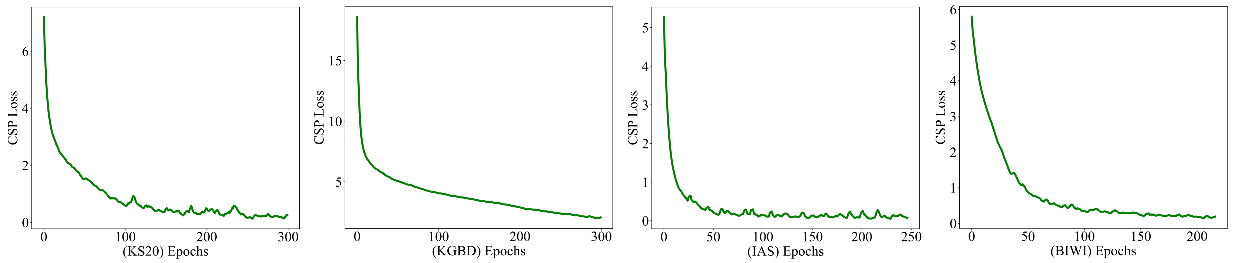


Figure 4: The combinatorial skeleton prototype learning (CSP) loss ($\mathcal{L}_{\text{CSP}}$) curves on different training datasets.

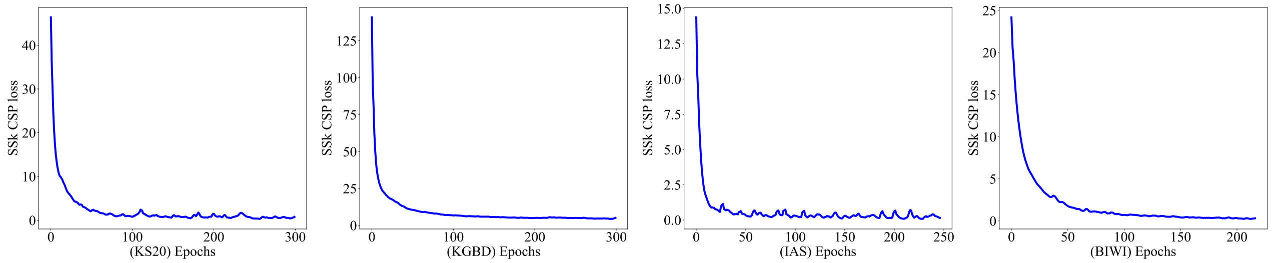


Figure 5: The sub-skeleton (SSk) level combinatorial skeleton prototype learning (CSP) loss ($\mathcal{L}_{\text{CSP}}^{ssk}$) curves on different training datasets.

Prompted Reconstruction for Person Re-Identification. In *Proceedings of the IEEE/CVF Conference on Computer Vision and Pattern Recognition (CVPR)*.

Rao, H.; Wang, S.; Hu, X.; Tan, M.; Da, H.; Cheng, J.; and Hu, B. 2020. Self-Supervised Gait Encoding with Locality-Aware Attention for Person Re-Identification. In *International Joint Conference on Artificial Intelligence (IJCAI)*, volume 1, 898–905.

Rao, H.; Wang, S.; Hu, X.; Tan, M.; Guo, Y.; Cheng, J.; Liu, X.; and Hu, B. 2021b. A self-supervised gait encoding approach with locality-awareness for 3D skeleton based person re-identification. *IEEE Transactions on Pattern Analysis and Machine Intelligence*, 44(10): 6649–6666.

Rao, H.; Xu, S.; Hu, X.; Cheng, J.; and Hu, B. 2021c. Multi-Level Graph Encoding with Structural-Collaborative Relation Learning for Skeleton-Based Person Re-Identification. In *International Joint Conference on Artificial Intelligence (IJCAI)*, 973–980.

Shotton, J.; Fitzgibbon, A.; Cook, M.; Sharp, T.; Finocchio, M. J.; Moore, R.; Kipman, A. A.; and Blake, A. 2011. Real-time human pose recognition in parts from single depth images. In *Proceedings of the IEEE/CVF Conference on Computer Vision and Pattern Recognition (CVPR)*, 1297–1304.

Yu, S.; Tan, D.; and Tan, T. 2006. A framework for evaluating the effect of view angle, clothing and carrying condition on gait recognition. In *International Conference on Pattern Recognition (ICPR)*, volume 4, 441–444. IEEE.

Zhao, R.; Wang, K.; Su, H.; and Ji, Q. 2019. Bayesian Graph Convolution LSTM for Skeleton Based Action Recognition. In *Proceedings of the IEEE/CVF International Conference on Computer Vision (ICCV)*, 6882–6892.

Zheng, L.; Shen, L.; Tian, L.; Wang, S.; Wang, J.; and Tian, Q. 2015. Scalable person re-identification: A benchmark. In *Proceedings of the IEEE/CVF International Conference on Computer Vision (ICCV)*, 1116–1124.

Zhong, Z.; Zheng, L.; Cao, D.; and Li, S. 2017. Re-ranking person re-identification with k-reciprocal encoding. In *Proceedings of the IEEE/CVF Conference on Computer Vision and Pattern Recognition (CVPR)*, 1318–1327.

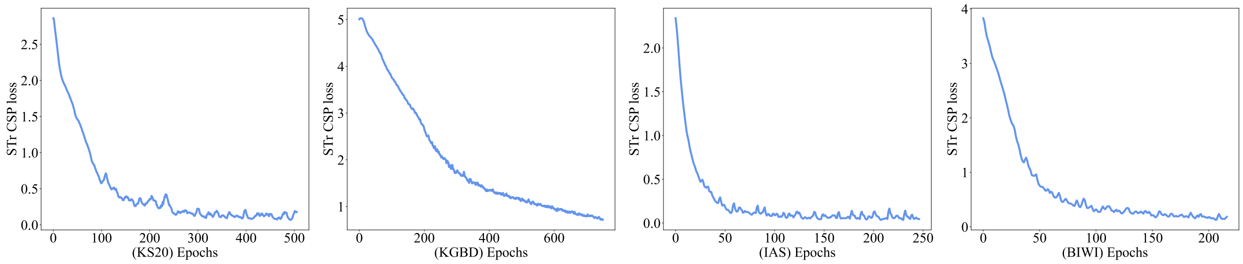


Figure 6: The sub-tracklet (STr) level combinatorial skeleton prototype learning (CSP) loss ($\mathcal{L}_{\text{CSP}}^{str}$) curves on different training datasets.

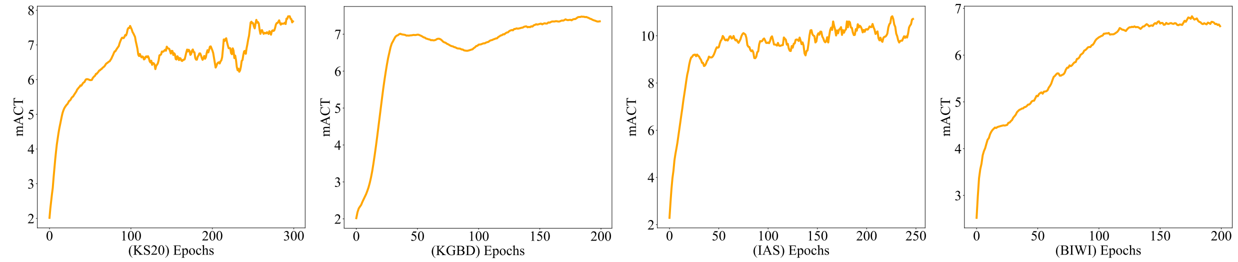


Figure 7: The mean intra-class tightness (mACT) of skeleton representations learned by our approach on different training datasets.

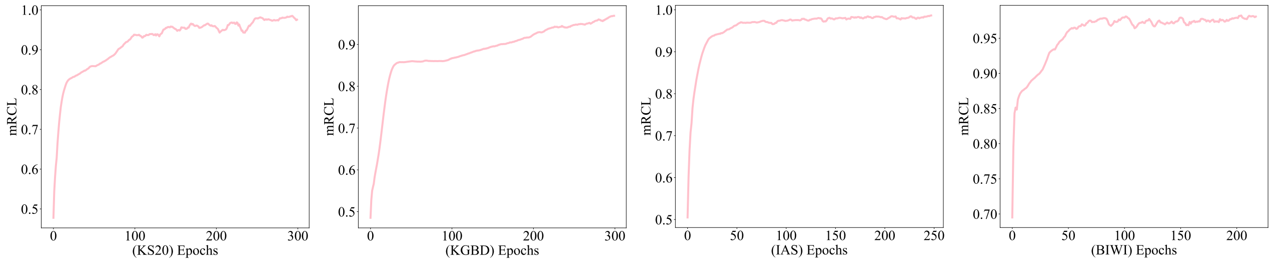


Figure 8: The mean inter-class looseness (mRCL) of skeleton representations learned by our approach on different training datasets.

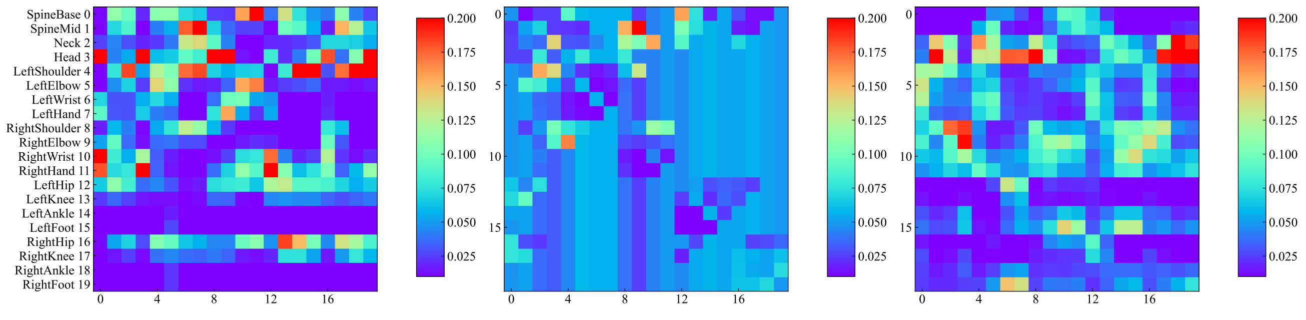


(a) (b) (c)

Figure 9: Visualization of relational value between body-joint nodes for testing (probe) skeletons in IAS-A. (a)-(c) represent the relations learned by the $1^{st}$ (HSM guided relations), $4^{th}$ (GCM guided relations), and $8^{th}$ (non-motif-guided full relations) heads. Note that the abscissa and ordinate denote indices of nodes (see Sec. A.4).

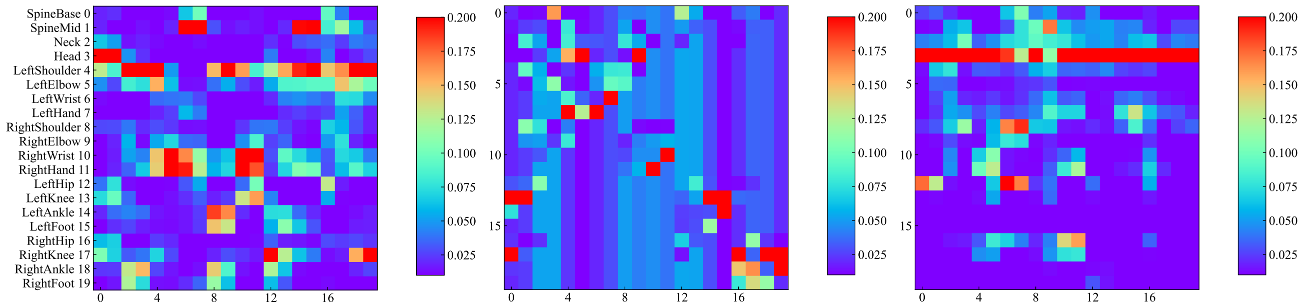


(a) (b) (c)

Figure 10: Visualization of relational value between body-joint nodes for testing (probe) skeletons in IAS-B. (a)-(c) represent the relations learned by the $1^{st}$ (HSM guided relations), $4^{th}$ (GCM guided relations), and $8^{th}$ (non-motif-guided full relations) heads. Note that the abscissa and ordinate denote indices of nodes (see Sec. A.4).

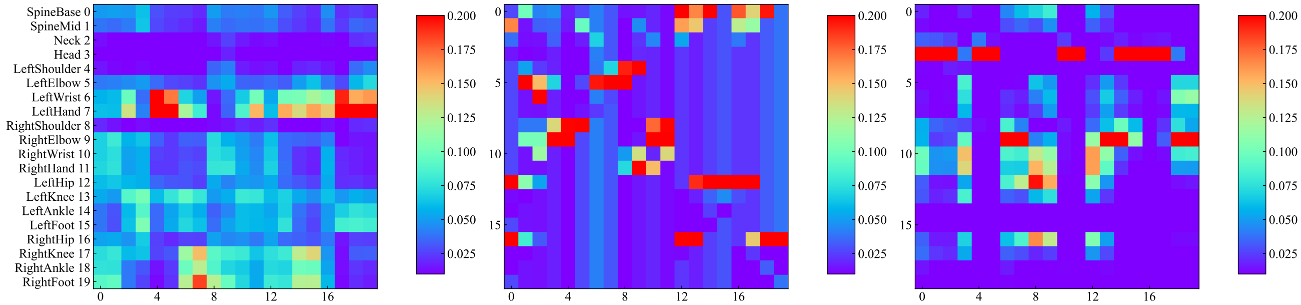


(a) (b) (c)

Figure 11: Visualization of relational value between body-joint nodes for testing (probe) skeletons in BIWI-S. (a)-(c) represent the relations learned by the $1^{st}$ (HSM guided relations), $4^{th}$ (GCM guided relations), and $8^{th}$ (non-motif-guided full relations) heads. Note that the abscissa and ordinate denote indices of nodes (see Sec. A.4).

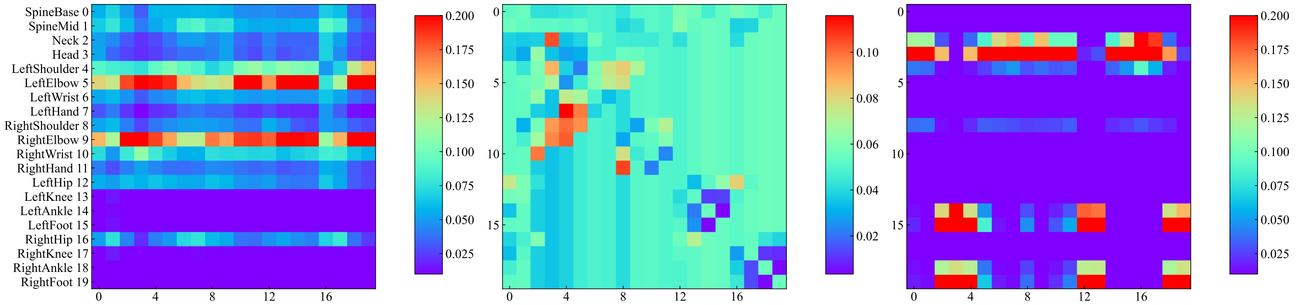


(a) (b) (c)

Figure 12: Visualization of relational value between body-joint nodes for testing (probe) skeletons in BIWI-W. (a)-(c) represent the relations learned by the $1^{st}$ (HSM guided relations), $4^{th}$ (GCM guided relations), and $8^{th}$ (non-motif-guided full relations) heads. Note that the abscissa and ordinate denote indices of nodes (see Sec. A.4).

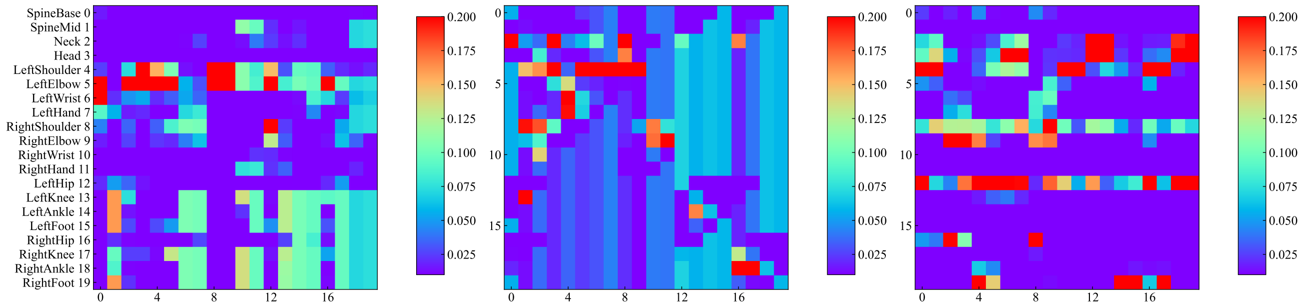


(a) (b) (c)

Figure 13: Visualization of relational value between body-joint nodes for testing (probe) skeletons in KGBD. (a)-(c) represent the relations learned by the $1^{st}$ (HSM guided relations), $4^{th}$ (GCM guided relations), and $8^{th}$ (non-motif-guided full relations) heads. Note that the abscissa and ordinate denote indices of nodes (see Sec. A.4).

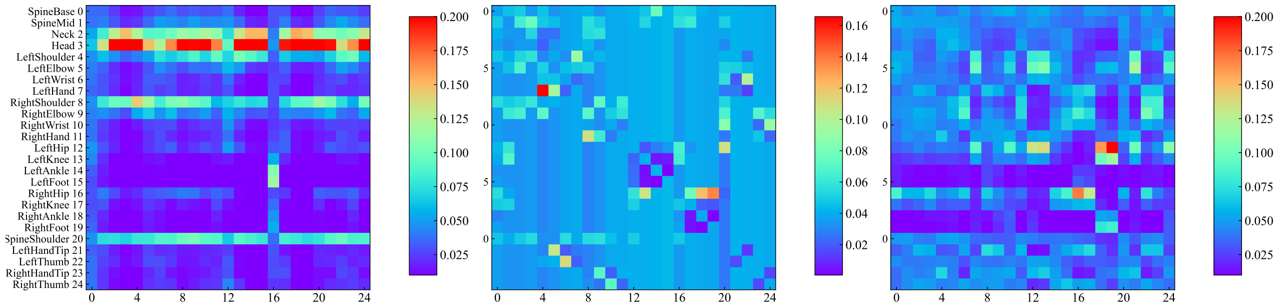


(a) (b) (c)

Figure 14: Visualization of relational value between body-joint nodes for testing (probe) skeletons in KS20. (a)-(c) represent the relations learned by the $1^{st}$ (HSM guided relations), $4^{th}$ (GCM guided relations), and $8^{th}$ (non-motif-guided full relations) heads. Note that the abscissa and ordinate denote indices of nodes (see Sec. A.4).

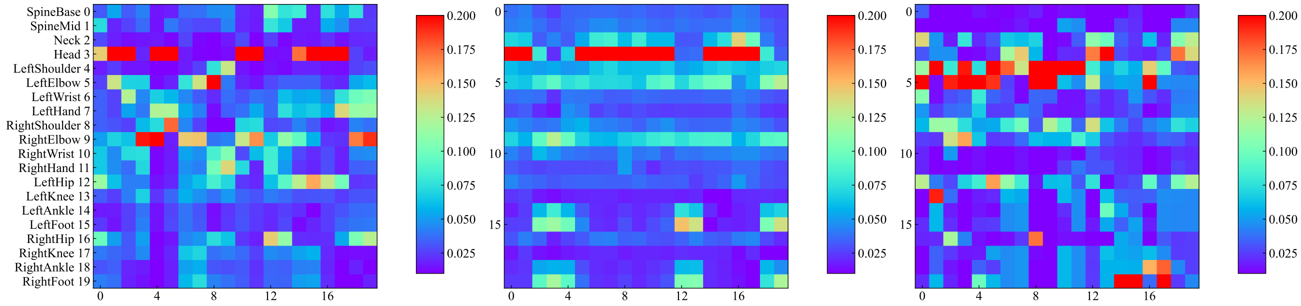


(a) (b) (c)

Figure 15: Visualization of mean relational value (over all relation heads) between body-joint nodes for testing skeletons in BIWI-S (a), BIWI-W (b), and KGBD (c). Note that the abscissa and ordinate denote indices of nodes (see Sec. A.4).

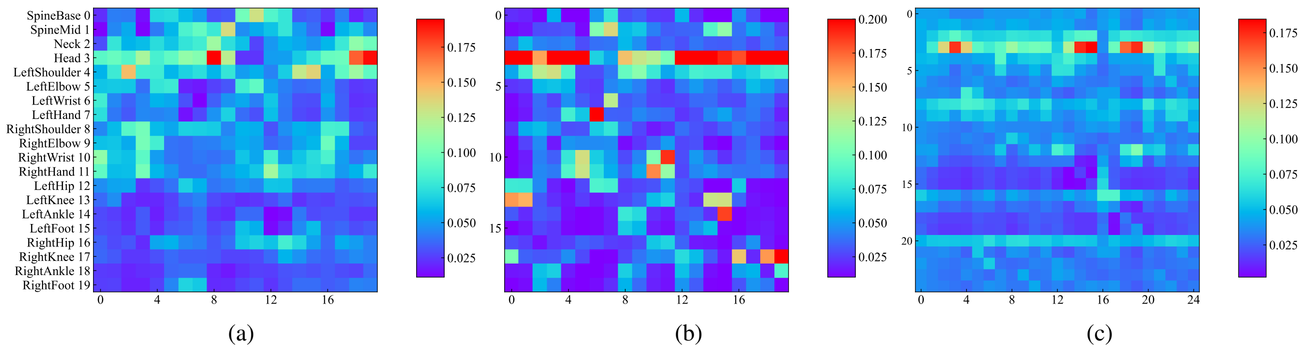


Figure 16: Visualization of mean relational value (over all relation heads) between body-joint nodes for testing skeletons in IAS-A (a), IAS-B (b), and KS20 (c). Note that the abscissa and ordinate denote indices of nodes (see Sec. A.4).

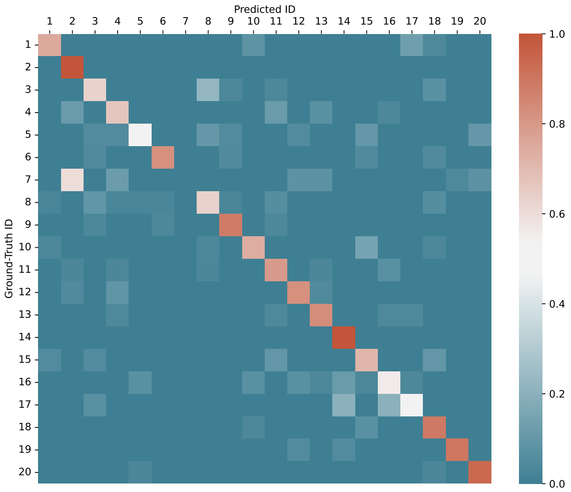


(a) Confusion Matrix on KS20

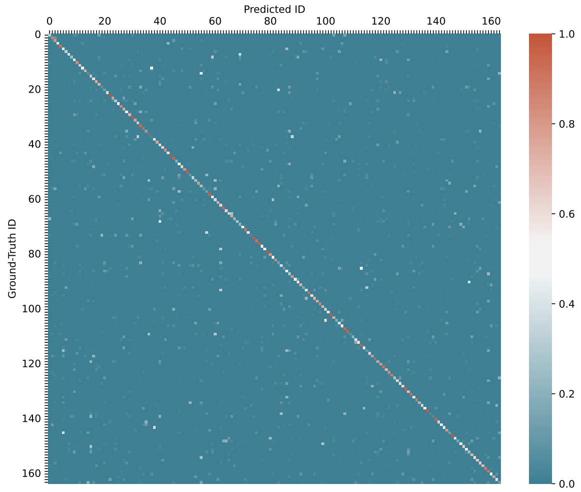


(b) Confusion Matrix on KGBD

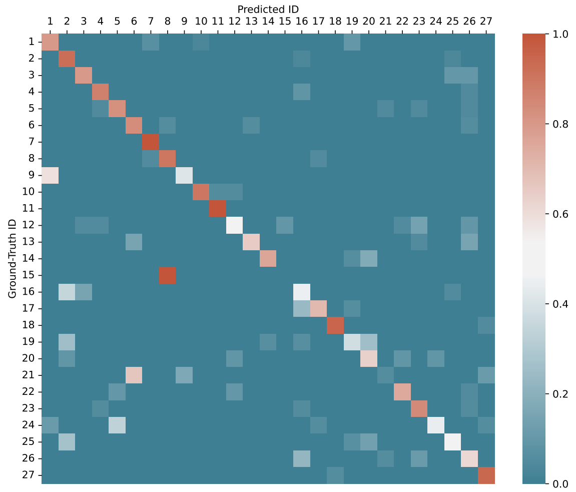


(c) Confusion Matrix on BIWI-S

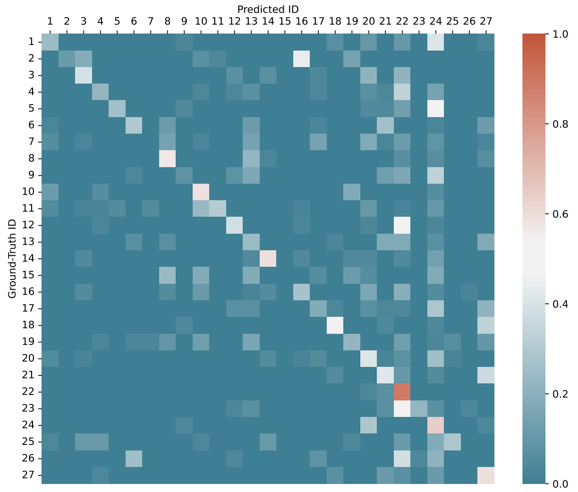


(d) Confusion Matrix on BIWI-W

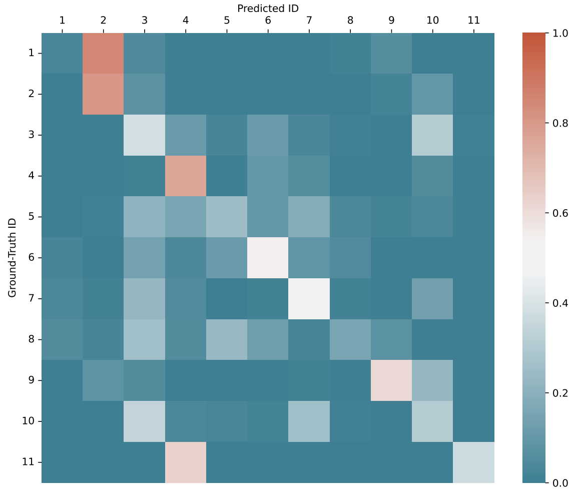


(e) Confusion Matrix on IAS-A

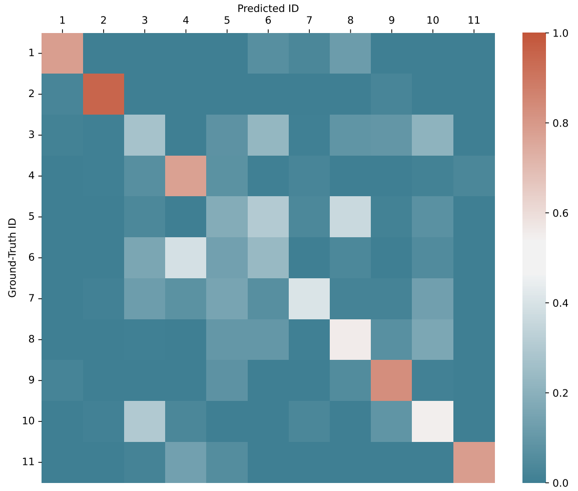


(f) Confusion Matrix on IAS-B

Figure 17: Visualization of confusion matrices on KS20 (a), KGBD (b), BIWI-S (c), BIWI-W (d), IAS-A (e), and IAS-B (f) when using the Rank-1 matching. Note that abscissa and ordinate denote the predicted and ground-truth identities, respectively. The position in the $a^{th}$ row and $b^{th}$ column indicates that the testing samples belonging to the $a^{th}$ identity is predicted as the $b^{th}$ identity, while the corresponding value is the proportion of such samples to the same-identity samples in the testing set.
